# Supplementary material for: SFlexRCA: Lightweight, Scalable, and Flexible Root Cause Analysis for IIoT Edge Systems
Source: arXiv:2610.04893 source file (2026-10-04)
Supplement: Supplementary file 1 [file Appendix.tex]

\section{Appendix}




\section{Results}
\subsection{RQ1}
\subsubsection{SMD dataset}

\begin{tabular}{l l l | rrrr | rrrr}
\toprule
& & & \multicolumn{4}{c}{Accuracy Metrics} & \multicolumn{4}{c}{Efficiency Metrics} \\
Architecture & Params & Win & AC@1 & AC@3 & Avg@10 & MRR & Inf. Time & Peak Mem & Tr. Epoch & Tr. Thr. \\
\midrule

\rowcolor{gray!20} \multicolumn{11}{c}{\textbf{SMD}} \\
baro & 0.000M & 4 & \textbf{0.520\tiny{±0.000}} & \textbf{0.463\tiny{±0.000}} & \textbf{0.537\tiny{±0.000}} & \textbf{0.633\tiny{±0.000}} & 0.000\tiny{±0.000} & 0.000\tiny{±0.000} & 0.000\tiny{±0.000} & 0.000\tiny{±0.000} \\
torai & 0.000M & 4 & \underline{0.489\tiny{±0.000}} & 0.432\tiny{±0.000} & \underline{0.504\tiny{±0.000}} & \underline{0.608\tiny{±0.000}} & 0.000\tiny{±0.000} & 0.000\tiny{±0.000} & 0.000\tiny{±0.000} & 0.000\tiny{±0.000} \\
SFlexRCA & 0.050M & 4 & 0.456\tiny{±0.029} & \underline{0.450\tiny{±0.018}} & 0.471\tiny{±0.019} & 0.586\tiny{±0.028} & 0.086\tiny{±0.030} & 18.458\tiny{±0.000} & 4.763\tiny{±1.163} & 30824.760\tiny{±6606.704} \\
CUTS_PLUS & 0.079M & 4 & 0.437\tiny{±0.014} & 0.421\tiny{±0.012} & 0.443\tiny{±0.013} & 0.403\tiny{±0.267} & 0.092\tiny{±0.049} & 17.913\tiny{±0.000} & \underline{26.736\tiny{±8.933}} & 5652.077\tiny{±1584.010} \\
SFlexRCA & 0.050M & 6 & 0.406\tiny{±0.022} & 0.387\tiny{±0.004} & 0.410\tiny{±0.005} & 0.537\tiny{±0.007} & 0.069\tiny{±0.001} & 18.569\tiny{±0.000} & 3.336\tiny{±0.039} & 28315.509\tiny{±329.092} \\
cLSTM & 3.3M & 4 & 0.397\tiny{±0.012} & 0.339\tiny{±0.004} & 0.383\tiny{±0.006} & 0.374\tiny{±0.241} & 0.099\tiny{±0.040} & \underline{70.218\tiny{±0.000}} & 26.214\tiny{±9.715} & 5845.927\tiny{±1785.752} \\
CUTS_PLUS & 0.079M & 6 & 0.385\tiny{±0.008} & 0.362\tiny{±0.025} & 0.372\tiny{±0.022} & 0.373\tiny{±0.222} & 0.076\tiny{±0.009} & 17.915\tiny{±0.000} & \textbf{27.671\tiny{±8.063}} & 3587.302\tiny{±895.006} \\
SFlexRCA & 0.056M & 20 & 0.368\tiny{±0.048} & 0.317\tiny{±0.008} & 0.335\tiny{±0.020} & 0.479\tiny{±0.040} & \textbf{0.102\tiny{±0.026}} & 19.340\tiny{±0.000} & 2.428\tiny{±0.053} & 11674.890\tiny{±253.739} \\
baro & 0.000M & 20 & 0.332\tiny{±0.000} & 0.336\tiny{±0.000} & 0.386\tiny{±0.000} & 0.465\tiny{±0.000} & 0.000\tiny{±0.000} & 0.000\tiny{±0.000} & 0.000\tiny{±0.000} & 0.000\tiny{±0.000} \\
CUTS_PLUS & 0.079M & 20 & 0.329\tiny{±nan} & 0.311\tiny{±nan} & 0.331\tiny{±nan} & 0.450\tiny{±nan} & 0.080\tiny{±nan} & 17.925\tiny{±nan} & 25.308\tiny{±nan} & 1119.625\tiny{±nan} \\
CUTS_PLUS & 0.079M & 10 & 0.326\tiny{±nan} & 0.314\tiny{±nan} & 0.334\tiny{±nan} & 0.447\tiny{±nan} & 0.064\tiny{±nan} & 17.917\tiny{±nan} & 23.816\tiny{±nan} & 2379.538\tiny{±nan} \\
baro & 0.000M & 6 & 0.314\tiny{±0.000} & 0.319\tiny{±0.000} & 0.361\tiny{±0.000} & 0.438\tiny{±0.000} & 0.000\tiny{±0.000} & 0.000\tiny{±0.000} & 0.000\tiny{±0.000} & 0.000\tiny{±0.000} \\
baro & 0.000M & 10 & 0.314\tiny{±0.000} & 0.310\tiny{±0.000} & 0.341\tiny{±0.000} & 0.432\tiny{±0.000} & 0.000\tiny{±0.000} & 0.000\tiny{±0.000} & 0.000\tiny{±0.000} & 0.000\tiny{±0.000} \\
SFlexRCA & 0.052M & 10 & 0.312\tiny{±0.076} & 0.318\tiny{±0.071} & 0.319\tiny{±0.065} & 0.429\tiny{±0.079} & 0.085\tiny{±0.010} & 18.789\tiny{±0.000} & 2.783\tiny{±0.048} & 20363.813\tiny{±349.414} \\
cLSTM & 3.3M & 6 & 0.310\tiny{±0.062} & 0.272\tiny{±0.014} & 0.305\tiny{±0.011} & 0.320\tiny{±0.207} & 0.078\tiny{±0.024} & 69.617\tiny{±0.000} & 16.881\tiny{±4.817} & 5868.783\tiny{±1438.138} \\
torai & 0.000M & 6 & 0.305\tiny{±0.009} & 0.281\tiny{±0.005} & 0.326\tiny{±0.004} & 0.419\tiny{±0.006} & 0.000\tiny{±0.000} & 0.000\tiny{±0.000} & 0.000\tiny{±0.000} & 0.000\tiny{±0.000} \\
torai & 0.000M & 10 & 0.277\tiny{±0.009} & 0.261\tiny{±0.006} & 0.286\tiny{±0.004} & 0.376\tiny{±0.007} & 0.000\tiny{±0.000} & 0.000\tiny{±0.000} & 0.000\tiny{±0.000} & 0.000\tiny{±0.000} \\
torai & 0.000M & 20 & 0.257\tiny{±0.005} & 0.263\tiny{±0.003} & 0.285\tiny{±0.001} & 0.355\tiny{±0.002} & 0.000\tiny{±0.000} & 0.000\tiny{±0.000} & 0.000\tiny{±0.000} & 0.000\tiny{±0.000} \\
cLSTM & 3.3M & 20 & 0.243\tiny{±0.029} & 0.235\tiny{±0.032} & 0.265\tiny{±0.024} & 0.309\tiny{±0.103} & \underline{0.101\tiny{±0.019}} & 69.773\tiny{±0.000} & 6.393\tiny{±0.518} & 4454.098\tiny{±361.495} \\
GVAR & 0.6M & 4 & 0.239\tiny{±0.017} & 0.234\tiny{±0.008} & 0.253\tiny{±0.010} & 0.354\tiny{±0.012} & 0.087\tiny{±0.025} & 26.992\tiny{±0.000} & 3.777\tiny{±1.705} & \textbf{42055.385\tiny{±15090.007}} \\
cLSTM & 3.3M & 10 & 0.210\tiny{±0.007} & 0.225\tiny{±0.010} & 0.260\tiny{±0.000} & 0.259\tiny{±0.135} & 0.080\tiny{±0.014} & 69.661\tiny{±0.000} & 10.071\tiny{±1.815} & 5740.322\tiny{±940.516} \\
GVAR & 1.0M & 6 & 0.203\tiny{±0.004} & 0.214\tiny{±0.010} & 0.244\tiny{±0.012} & 0.334\tiny{±0.010} & 0.068\tiny{±0.002} & 33.348\tiny{±0.000} & 2.454\tiny{±0.040} & \underline{38498.420\tiny{±624.417}} \\
GVAR & 1.9M & 10 & 0.200\tiny{±0.030} & 0.210\tiny{±0.034} & 0.235\tiny{±0.024} & 0.326\tiny{±0.035} & 0.074\tiny{±0.016} & 46.060\tiny{±0.000} & 2.133\tiny{±0.019} & 26573.275\tiny{±242.183} \\
GVAR & 3.9M & 20 & 0.146\tiny{±0.017} & 0.173\tiny{±0.011} & 0.198\tiny{±0.013} & 0.288\tiny{±0.008} & 0.099\tiny{±0.017} & \textbf{77.840\tiny{±0.000}} & 2.450\tiny{±0.292} & 11677.383\tiny{±1405.884} \\
rcd & 0.000M & 4 & 0.003\tiny{±0.000} & 0.148\tiny{±0.000} & 0.306\tiny{±0.000} & 0.410\tiny{±0.000} & 0.000\tiny{±0.000} & 0.000\tiny{±0.000} & 0.000\tiny{±0.000} & 0.000\tiny{±0.000} \\
rcd & 0.000M & 6 & 0.003\tiny{±0.000} & 0.148\tiny{±0.000} & 0.306\tiny{±0.000} & 0.410\tiny{±0.000} & 0.000\tiny{±0.000} & 0.000\tiny{±0.000} & 0.000\tiny{±0.000} & 0.000\tiny{±0.000} \\
rcd & 0.000M & 10 & 0.003\tiny{±0.000} & 0.148\tiny{±0.000} & 0.306\tiny{±0.000} & 0.410\tiny{±0.000} & 0.000\tiny{±0.000} & 0.000\tiny{±0.000} & 0.000\tiny{±0.000} & 0.000\tiny{±0.000} \\
rcd & 0.000M & 20 & 0.003\tiny{±0.000} & 0.148\tiny{±0.000} & 0.306\tiny{±0.000} & 0.410\tiny{±0.000} & 0.000\tiny{±0.000} & 0.000\tiny{±0.000} & 0.000\tiny{±0.000} & 0.000\tiny{±0.000} \\
\bottomrule
\end{tabular}


\subsubsection{AIOps dataset}
\begin{tabular}{l l l | rrrr | rrrr}
\toprule
& & & \multicolumn{4}{c}{Accuracy Metrics} & \multicolumn{4}{c}{Efficiency Metrics} \\
Architecture & Params & Win & AC@1 & AC@3 & Avg@10 & MRR & Inf. Time & Peak Mem & Tr. Epoch & Tr. Thr. \\
\midrule

\rowcolor{gray!20} \multicolumn{11}{c}{\textbf{AIOPS}} \\
SFlexRCA & 0.2M & 20 & \textbf{0.368\tiny{±0.009}} & \textbf{0.429\tiny{±0.007}} & \textbf{0.467\tiny{±0.008}} & 0.435\tiny{±0.006} & 0.083\tiny{±0.036} & 21.462\tiny{±0.000} & 0.438\tiny{±0.068} & 10599.350\tiny{±1632.687} \\
baro & 0.000M & 20 & \underline{0.348\tiny{±0.000}} & 0.404\tiny{±0.000} & 0.435\tiny{±0.000} & 0.208\tiny{±0.241} & 0.000\tiny{±0.000} & 0.000\tiny{±0.000} & 0.000\tiny{±0.000} & 0.000\tiny{±0.000} \\
SFlexRCA & 0.2M & 16 & 0.345\tiny{±0.073} & \underline{0.409\tiny{±0.064}} & \underline{0.442\tiny{±0.075}} & 0.413\tiny{±0.066} & 0.090\tiny{±0.032} & 21.266\tiny{±0.000} & 0.359\tiny{±0.060} & 13041.722\tiny{±2016.567} \\
SFlexRCA & 0.2M & 12 & 0.338\tiny{±0.070} & 0.403\tiny{±0.061} & 0.434\tiny{±0.070} & 0.405\tiny{±0.065} & 0.103\tiny{±0.045} & 21.071\tiny{±0.000} & 0.291\tiny{±0.038} & 16024.476\tiny{±2055.323} \\
baro & 0.000M & 16 & 0.331\tiny{±0.000} & 0.392\tiny{±0.000} & 0.420\tiny{±0.000} & 0.202\tiny{±0.234} & 0.000\tiny{±0.000} & 0.000\tiny{±0.000} & 0.000\tiny{±0.000} & 0.000\tiny{±0.000} \\
baro & 0.000M & 12 & 0.317\tiny{±0.000} & 0.385\tiny{±0.000} & 0.410\tiny{±0.000} & 0.197\tiny{±0.211} & 0.000\tiny{±0.000} & 0.000\tiny{±0.000} & 0.000\tiny{±0.000} & 0.000\tiny{±0.000} \\
CUTS_PLUS & 0.2M & 16 & 0.293\tiny{±0.070} & 0.326\tiny{±0.005} & 0.339\tiny{±0.003} & 0.361\tiny{±0.049} & 0.087\tiny{±0.043} & 21.000\tiny{±0.000} & \underline{4.946\tiny{±1.663}} & 984.579\tiny{±330.964} \\
baro & 0.000M & 8 & 0.283\tiny{±0.000} & 0.365\tiny{±0.000} & 0.382\tiny{±0.000} & 0.184\tiny{±0.202} & 0.000\tiny{±0.000} & 0.000\tiny{±0.000} & 0.000\tiny{±0.000} & 0.000\tiny{±0.000} \\
torai & 0.000M & 16 & 0.281\tiny{±0.000} & 0.364\tiny{±0.000} & 0.380\tiny{±0.000} & \textbf{0.452\tiny{±0.000}} & 0.000\tiny{±0.000} & 0.000\tiny{±0.000} & 0.000\tiny{±0.000} & 0.000\tiny{±0.000} \\
cLSTM & 8.9M & 20 & 0.278\tiny{±0.043} & 0.311\tiny{±0.027} & 0.319\tiny{±0.018} & 0.326\tiny{±0.030} & 0.099\tiny{±0.029} & 162.228\tiny{±0.000} & 1.193\tiny{±0.247} & 3933.000\tiny{±815.371} \\
torai & 0.000M & 12 & 0.278\tiny{±0.000} & 0.354\tiny{±0.000} & 0.369\tiny{±0.000} & 0.445\tiny{±0.000} & 0.000\tiny{±0.000} & 0.000\tiny{±0.000} & 0.000\tiny{±0.000} & 0.000\tiny{±0.000} \\
torai & 0.000M & 20 & 0.274\tiny{±0.000} & 0.356\tiny{±0.000} & 0.377\tiny{±0.000} & \underline{0.446\tiny{±0.000}} & 0.000\tiny{±0.000} & 0.000\tiny{±0.000} & 0.000\tiny{±0.000} & 0.000\tiny{±0.000} \\
GVAR & 4.6M & 16 & 0.272\tiny{±0.016} & 0.314\tiny{±0.019} & 0.328\tiny{±0.009} & 0.341\tiny{±0.015} & 0.102\tiny{±0.025} & 87.923\tiny{±0.000} & 0.422\tiny{±0.146} & 12072.507\tiny{±5179.605} \\
cLSTM & 8.9M & 12 & 0.272\tiny{±0.015} & 0.313\tiny{±0.008} & 0.331\tiny{±0.009} & 0.328\tiny{±0.011} & 0.084\tiny{±0.029} & \underline{162.410\tiny{±0.000}} & 0.940\tiny{±0.296} & 5284.112\tiny{±1664.464} \\
GVAR & 3.4M & 12 & 0.268\tiny{±0.017} & 0.320\tiny{±0.011} & 0.333\tiny{±0.007} & 0.336\tiny{±0.013} & 0.079\tiny{±0.029} & 69.281\tiny{±0.000} & 0.299\tiny{±0.116} & 17287.904\tiny{±6673.818} \\
GVAR & 5.8M & 20 & 0.263\tiny{±0.007} & 0.306\tiny{±0.001} & 0.324\tiny{±0.002} & 0.337\tiny{±0.008} & 0.081\tiny{±0.045} & 106.564\tiny{±0.000} & 0.447\tiny{±0.231} & 11858.875\tiny{±6127.958} \\
CUTS_PLUS & 0.2M & 20 & 0.259\tiny{±0.031} & 0.296\tiny{±0.017} & 0.319\tiny{±0.000} & 0.328\tiny{±0.024} & \underline{0.116\tiny{±0.080}} & 21.003\tiny{±0.000} & \textbf{6.260\tiny{±2.101}} & 777.381\tiny{±260.887} \\
CUTS_PLUS & 0.2M & 8 & 0.257\tiny{±0.009} & 0.315\tiny{±0.011} & 0.334\tiny{±0.009} & 0.331\tiny{±0.011} & 0.114\tiny{±0.030} & 20.994\tiny{±0.000} & 2.397\tiny{±0.509} & 1986.725\tiny{±477.098} \\
torai & 0.000M & 8 & 0.257\tiny{±0.000} & 0.319\tiny{±0.000} & 0.336\tiny{±0.000} & 0.314\tiny{±0.209} & 0.000\tiny{±0.000} & 0.000\tiny{±0.000} & 0.000\tiny{±0.000} & 0.000\tiny{±0.000} \\
cLSTM & 8.9M & 16 & 0.253\tiny{±0.008} & 0.313\tiny{±0.014} & 0.329\tiny{±0.008} & 0.328\tiny{±0.013} & 0.081\tiny{±0.036} & \textbf{165.062\tiny{±0.000}} & 1.057\tiny{±0.293} & 4520.404\tiny{±1253.082} \\
SFlexRCA & 0.2M & 8 & 0.250\tiny{±0.090} & 0.373\tiny{±0.060} & 0.398\tiny{±0.068} & 0.380\tiny{±0.068} & 0.097\tiny{±0.037} & 20.876\tiny{±0.000} & 0.251\tiny{±0.057} & \underline{19053.284\tiny{±4613.487}} \\
CUTS_PLUS & 0.2M & 12 & 0.242\tiny{±0.028} & 0.309\tiny{±0.021} & 0.331\tiny{±0.012} & 0.320\tiny{±0.022} & 0.094\tiny{±0.030} & 20.997\tiny{±0.000} & 3.765\tiny{±0.869} & 1273.162\tiny{±338.075} \\
GVAR & 2.1M & 8 & 0.241\tiny{±0.032} & 0.298\tiny{±0.010} & 0.329\tiny{±0.003} & 0.317\tiny{±0.018} & \textbf{0.119\tiny{±0.076}} & 50.640\tiny{±0.000} & 0.252\tiny{±0.092} & \textbf{20337.329\tiny{±8613.897}} \\
cLSTM & 8.9M & 8 & 0.237\tiny{±0.008} & 0.303\tiny{±0.010} & 0.319\tiny{±0.007} & 0.302\tiny{±0.012} & 0.099\tiny{±0.038} & 161.122\tiny{±0.000} & 0.925\tiny{±0.304} & 5454.639\tiny{±2206.805} \\
rcd & 0.000M & 20 & 0.194\tiny{±0.000} & 0.274\tiny{±0.000} & 0.287\tiny{±0.000} & 0.302\tiny{±0.000} & 0.000\tiny{±0.000} & 0.000\tiny{±0.000} & 0.000\tiny{±0.000} & 0.000\tiny{±0.000} \\
rcd & 0.000M & 16 & 0.190\tiny{±0.000} & 0.271\tiny{±0.000} & 0.285\tiny{±0.000} & 0.299\tiny{±0.000} & 0.000\tiny{±0.000} & 0.000\tiny{±0.000} & 0.000\tiny{±0.000} & 0.000\tiny{±0.000} \\
rcd & 0.000M & 12 & 0.185\tiny{±0.000} & 0.267\tiny{±0.000} & 0.283\tiny{±0.000} & 0.295\tiny{±0.000} & 0.000\tiny{±0.000} & 0.000\tiny{±0.000} & 0.000\tiny{±0.000} & 0.000\tiny{±0.000} \\
rcd & 0.000M & 8 & 0.178\tiny{±0.000} & 0.262\tiny{±0.000} & 0.279\tiny{±0.000} & 0.289\tiny{±0.000} & 0.000\tiny{±0.000} & 0.000\tiny{±0.000} & 0.000\tiny{±0.000} & 0.000\tiny{±0.000} \\
\bottomrule
\end{tabular}




\subsection{GAIA dataset}

\begin{tabular}{l l l | rrrr | rrrr}
\toprule
& & & \multicolumn{4}{c}{Accuracy Metrics} & \multicolumn{4}{c}{Efficiency Metrics} \\
Architecture & Params & Win & AC@1 & AC@3 & Avg@10 & MRR & Inf. Time & Peak Mem & Tr. Epoch & Tr. Thr. \\
\midrule

\rowcolor{gray!20} \multicolumn{11}{c}{\textbf{GAIA}} \\
SFlexRCA & 0.2M & 12 & \textbf{0.280\tiny{±0.000}} & 0.282\tiny{±0.000} & 0.290\tiny{±0.000} & \textbf{0.382\tiny{±0.000}} & 0.094\tiny{±0.002} & 21.775\tiny{±0.000} & 6.262\tiny{±0.020} & 12741.875\tiny{±41.242} \\
cLSTM & 15.8M & 8 & \underline{0.257\tiny{±0.020}} & 0.248\tiny{±0.013} & 0.291\tiny{±0.056} & 0.337\tiny{±0.028} & 0.095\tiny{±0.001} & 276.261\tiny{±0.000} & \underline{22.548\tiny{±0.247}} & 5311.243\tiny{±58.197} \\
GVAR & 7.9M & 12 & 0.248\tiny{±0.041} & 0.244\tiny{±0.060} & 0.245\tiny{±0.057} & 0.310\tiny{±0.046} & 0.094\tiny{±0.007} & 140.911\tiny{±0.000} & 3.850\tiny{±0.384} & 20859.160\tiny{±2045.182} \\
cLSTM & 15.8M & 12 & 0.238\tiny{±0.053} & 0.228\tiny{±0.054} & 0.261\tiny{±0.056} & 0.342\tiny{±0.010} & 0.090\tiny{±0.009} & \textbf{282.792\tiny{±0.000}} & 19.294\tiny{±0.280} & 4135.792\tiny{±59.526} \\
cLSTM & 15.8M & 10 & 0.236\tiny{±0.055} & 0.225\tiny{±0.002} & 0.248\tiny{±0.023} & 0.310\tiny{±0.030} & 0.087\tiny{±0.009} & \underline{281.172\tiny{±0.000}} & 20.232\tiny{±0.092} & 4734.018\tiny{±21.505} \\
GVAR & 5.0M & 8 & 0.220\tiny{±0.053} & 0.232\tiny{±0.008} & 0.280\tiny{±0.023} & 0.336\tiny{±0.023} & 0.091\tiny{±0.009} & 96.772\tiny{±0.000} & 4.255\tiny{±0.243} & \textbf{28191.398\tiny{±1609.846}} \\
torai & 0.000M & 10 & 0.216\tiny{±0.007} & 0.217\tiny{±0.001} & 0.417\tiny{±0.001} & 0.376\tiny{±0.004} & 0.000\tiny{±0.000} & 0.000\tiny{±0.000} & 0.000\tiny{±0.000} & 0.000\tiny{±0.000} \\
torai & 0.000M & 8 & 0.215\tiny{±0.002} & 0.218\tiny{±0.005} & \textbf{0.418\tiny{±0.002}} & \underline{0.378\tiny{±0.004}} & 0.000\tiny{±0.000} & 0.000\tiny{±0.000} & 0.000\tiny{±0.000} & 0.000\tiny{±0.000} \\
torai & 0.000M & 12 & 0.214\tiny{±0.003} & 0.215\tiny{±0.003} & 0.417\tiny{±0.001} & 0.375\tiny{±0.002} & 0.000\tiny{±0.000} & 0.000\tiny{±0.000} & 0.000\tiny{±0.000} & 0.000\tiny{±0.000} \\
torai & 0.000M & 14 & 0.211\tiny{±0.003} & 0.215\tiny{±0.002} & \underline{0.417\tiny{±0.001}} & 0.374\tiny{±0.004} & 0.000\tiny{±0.000} & 0.000\tiny{±0.000} & 0.000\tiny{±0.000} & 0.000\tiny{±0.000} \\
SFlexRCA & 0.2M & 8 & 0.210\tiny{±0.075} & \underline{0.297\tiny{±0.022}} & 0.313\tiny{±0.026} & 0.367\tiny{±0.025} & \underline{0.107\tiny{±0.002}} & 21.452\tiny{±0.000} & 6.659\tiny{±0.030} & 17983.499\tiny{±81.546} \\
GVAR & 9.4M & 14 & 0.204\tiny{±0.032} & 0.257\tiny{±0.058} & 0.288\tiny{±0.065} & 0.316\tiny{±0.027} & 0.105\tiny{±0.004} & 164.346\tiny{±0.000} & 3.697\tiny{±0.159} & 18519.130\tiny{±799.776} \\
SFlexRCA & 0.2M & 10 & 0.203\tiny{±0.053} & \textbf{0.315\tiny{±0.013}} & 0.297\tiny{±0.007} & 0.347\tiny{±0.019} & \textbf{0.109\tiny{±0.005}} & 21.612\tiny{±0.000} & 6.408\tiny{±0.053} & 14945.710\tiny{±123.205} \\
cLSTM & 15.8M & 14 & 0.197\tiny{±0.004} & 0.237\tiny{±0.017} & 0.239\tiny{±0.018} & 0.298\tiny{±0.041} & 0.094\tiny{±0.011} & 271.329\tiny{±0.000} & 18.851\tiny{±0.229} & 3627.306\tiny{±44.013} \\
GVAR & 6.5M & 10 & 0.153\tiny{±0.034} & 0.243\tiny{±0.045} & 0.282\tiny{±0.008} & 0.298\tiny{±0.038} & 0.100\tiny{±0.005} & 118.906\tiny{±0.000} & 4.038\tiny{±0.273} & \underline{23772.401\tiny{±1609.460}} \\
CUTS_PLUS & 0.3M & 8 & 0.151\tiny{±nan} & 0.223\tiny{±nan} & 0.311\tiny{±nan} & 0.317\tiny{±nan} & 0.080\tiny{±nan} & 21.654\tiny{±nan} & \textbf{91.393\tiny{±nan}} & 1310.304\tiny{±nan} \\
baro & 0.000M & 10 & 0.143\tiny{±0.000} & 0.150\tiny{±0.000} & 0.196\tiny{±0.000} & 0.258\tiny{±0.000} & 0.000\tiny{±0.000} & 0.000\tiny{±0.000} & 0.000\tiny{±0.000} & 0.000\tiny{±0.000} \\
baro & 0.000M & 12 & 0.143\tiny{±0.000} & 0.148\tiny{±0.000} & 0.194\tiny{±0.000} & 0.256\tiny{±0.000} & 0.000\tiny{±0.000} & 0.000\tiny{±0.000} & 0.000\tiny{±0.000} & 0.000\tiny{±0.000} \\
baro & 0.000M & 14 & 0.143\tiny{±0.000} & 0.142\tiny{±0.000} & 0.193\tiny{±0.000} & 0.254\tiny{±0.000} & 0.000\tiny{±0.000} & 0.000\tiny{±0.000} & 0.000\tiny{±0.000} & 0.000\tiny{±0.000} \\
baro & 0.000M & 8 & 0.140\tiny{±0.000} & 0.149\tiny{±0.000} & 0.197\tiny{±0.000} & 0.257\tiny{±0.000} & 0.000\tiny{±0.000} & 0.000\tiny{±0.000} & 0.000\tiny{±0.000} & 0.000\tiny{±0.000} \\
rcd & 0.000M & 8 & 0.140\tiny{±0.000} & 0.171\tiny{±0.000} & 0.218\tiny{±0.000} & 0.253\tiny{±0.000} & 0.000\tiny{±0.000} & 0.000\tiny{±0.000} & 0.000\tiny{±0.000} & 0.000\tiny{±0.000} \\
rcd & 0.000M & 10 & 0.140\tiny{±0.000} & 0.171\tiny{±0.000} & 0.218\tiny{±0.000} & 0.253\tiny{±0.000} & 0.000\tiny{±0.000} & 0.000\tiny{±0.000} & 0.000\tiny{±0.000} & 0.000\tiny{±0.000} \\
rcd & 0.000M & 12 & 0.140\tiny{±0.000} & 0.171\tiny{±0.000} & 0.218\tiny{±0.000} & 0.253\tiny{±0.000} & 0.000\tiny{±0.000} & 0.000\tiny{±0.000} & 0.000\tiny{±0.000} & 0.000\tiny{±0.000} \\
rcd & 0.000M & 14 & 0.140\tiny{±0.000} & 0.171\tiny{±0.000} & 0.218\tiny{±0.000} & 0.253\tiny{±0.000} & 0.000\tiny{±0.000} & 0.000\tiny{±0.000} & 0.000\tiny{±0.000} & 0.000\tiny{±0.000} \\
SFlexRCA & 0.2M & 14 & 0.120\tiny{±nan} & 0.221\tiny{±nan} & 0.211\tiny{±nan} & 0.257\tiny{±nan} & 0.088\tiny{±nan} & 21.938\tiny{±nan} & 6.126\tiny{±nan} & 11160.292\tiny{±nan} \\
\bottomrule
\end{tabular}
