# Supplementary material for: SFlexRCA: Lightweight, Scalable, and Flexible Root Cause Analysis for IIoT Edge Systems
Source: arXiv:2610.04893 source file (2026-10-04)
Supplement: Supplementary file 2 [file Appendix_old.tex]

\section{Appendix}





\subsection{Related Works}

\begin{table}[H]
	\centering
	\renewcommand{\arraystretch}{1.25}
	\setlength{\tabcolsep}{2pt}
	\caption{Related Works Comparison of Generic Time Series Models and Root Cause Analysis Methods}
	\begin{tabular}{|p{3.5cm}|p{2.8cm}|p{3.5cm}|p{1.8cm}|p{4.5cm}|}
		\hline
		\textbf{Method} & \textbf{Graph Structure} & \textbf{Attention} & \small{\textbf{Interpretable}} & \textbf{Key Strengths} \\ \hline
		
		\multicolumn{5}{|l|}{\cellcolor{gray!90} \textbf{Generic Time Series Models}} \\ \cline{2-5}
		& \multicolumn{4}{|l|}{\cellcolor{lightgray} \textbf{Time Domain}} \\ \hline
		iTransformer~\cite{itransformer} & \xmark & \cmark (Linear Self-Attn) & \xmark & Efficient for long sequences; scalable forecasting \\ \hline
		
		& \multicolumn{4}{|l|}{\cellcolor{lightgray} \textbf{Frequency Domain}} \\ \hline
		FEDformer~\cite{fedformer} & \xmark & \cmark (Sparse Fourier Attn) & \xmark & Captures periodic patterns; reduced complexity \\ \hline
		FITS~\cite{276-Fits} & \xmark & \xmark (Frequency MLP) & \xmark & High-resolution freq modeling; compact design \\ \hline
		
		& \multicolumn{4}{|l|}{\cellcolor{lightgray} \textbf{Time--Frequency Domain}} \\ \hline
		CrossFuN~\cite{290-crosstimefreq-CrossFun} & \xmark & \xmark (simple Time--Freq fusion) & \xmark & Fuses temporal and spectral info \\ \hline
		DeAnomaly~\cite{289-crosstimefreq-DeAnomaly} & \cmark (Graph) & \cmark (Cross Time--Freq Attn) & \xmark & Robust to noise; joint graph + time--freq fusion \\ \hline
		
		\multicolumn{5}{|l|}{\cellcolor{gray!90} \textbf{Root Cause Analysis Models}} \\ \cline{2-5}
		& \multicolumn{4}{|l|}{\cellcolor{lightgray} \textbf{Topology-Based Graph Methods}} \\ \hline
		MonitorRank~\cite{292-kim2013rcd} & \cmark (Call Graph) & \xmark & \xmark & PageRank-style ranking; interpretable \\ \hline
		MicroRCA~\cite{292-wu2020microrca} & \cmark (Topology) & \xmark & \xmark & Random walk scoring on anomalous subgraphs \\ \hline
		
		& \multicolumn{4}{|l|}{\cellcolor{lightgray} \textbf{Classical Statistical Techniques}} \\ \hline
		$\epsilon$-Diagnosis~\cite{286-Shan2019-EpsilonDiagnosis} & \xmark & \xmark & \xmark & Lightweight; interpretable; efficient \\ \hline
		N-Sigma~\cite{283-li2022-nsigma} & \xmark & \xmark & \xmark & Simple thresholding; effective for small anomalies \\ \hline
		BARO~\cite{283-root-bayes} & \xmark & \xmark & \xmark & Bayesian change-point detection; robust scoring \\ \hline
		
		& \multicolumn{4}{|l|}{\cellcolor{lightgray} \textbf{Causal Inference and Graph Neural Methods}} \\ \hline
		GVAR~\cite{GVAR} & \xmark & \xmark (Time MLP) & \cmark & Infers nonlinear Granger causality; interpretable causal effects in time series \\ \hline
		CORAL~\cite{CORAL} & \cmark (Disentangled Causal Graph) & \xmark & \cmark & Incremental online RCA; captures state-invariant and dependent dependencies \\ \hline
		AERCA~\cite{285-encoder-decoder} & \xmark & \xmark (Time MLP) & \cmark & Models interventions; interpretable \\ \hline
		\rowcolor{green!20} 
		Ours (CrGSTA) & \cmark (Graph Attn) & \cmark (Spatio-Temporal Cross Time-Freq Attn) & \cmark & Scalable; captures long-range dependencies; hybrid domain; GNN+Attn \\ \hline
	\end{tabular}
	\label{tab:rca_comparison}
\end{table}
In this section we provide a comparison of various Root Cause Analysis (RCA) and Anomaly Detection approaches in Table~\ref{tab:rca_comparison}. The table categorizes methods based on their graph structure, attention mechanisms, interpretability, and key strengths. This comparison highlights the unique features and advantages of each approach, providing a comprehensive overview of the landscape in this research area.


\subsection{Model}
In this section, we provide a detailed illustration of our proposed CrGSTA architecture in Figure~\ref{fig:SpectoGraphNet_detailed}. This figure visually represents the key components and data flow within the model, highlighting the loss functions, and the same graph structure used across time slices for clarity, and similarly the another single graph used across frequency slices. 
\begin{figure}[H]
	\centering
	\includegraphics[width=\textwidth]{Images/CrGSTA.pdf}
	\caption{CrGSTA: Time-Frequency Cross-Attention Graph Spatio-Temporal Autoencoder}
	\label{fig:SpectoGraphNet_detailed}
\end{figure}




\subsection{Intuitive Explanation of Model Equations}
\label{appendix:model_equations}
\subsubsection{Encoder Equations}

\textbf{Windowing.}
\begin{equation}
\mathbf{W}_t = (\mathbf{x}_{t-K+1}, \dots, \mathbf{x}_t)
\end{equation}
This extracts a sliding window of past observations. This allows the model to capture temporal dependencies over the recent history of the multivariate time series.

\textbf{Base Spatial Graph.}
\begin{equation}
\mathbf{H}^\text{base}_{t-k} = \text{GNN}(\mathbf{x}_{t-k})
\end{equation}
This computes pairwise interactions between variables at each lag. Using a graph neural network (GNN) enables the model to learn complex relationships among variables, which is crucial for identifying causal influences in multivariate data.

\textbf{Time-Domain Attention.}
\begin{equation}
\mathbf{A}^\text{time}_t = \text{TemporalAttn}([\mathbf{H}^\text{base}_{t-1:\,t-K}])
\end{equation}
This assigns attention weights to past time steps. This temporal attention mechanism allows the model to focus on the most relevant historical information when inferring exogenous variables.

\textbf{Frequency-Domain Attention.}
\begin{equation}
\mathbf{A}^\text{freq}_t = \text{TemporalAttn}([\mathbf{H}^\text{freq}_1,\dots,\mathbf{H}^\text{freq}_F])
\end{equation}
This assigns attention weights to frequency components. Studying the frequency domain helps capture periodic patterns and anomalies that may not be evident in the time domain alone. Similar to temporal attention, this mechanism helps the model identify important spectral features that may indicate anomalies or causal factors.

\textbf{Cross-Attention Fusion.}
\begin{equation}
\tilde{\mathbf{H}}^\text{time} = \text{CrossAttn}(\mathbf{A}^\text{time}_t, \mathbf{A}^\text{freq}_t)
\end{equation}
This mixes information between time and frequency. Mixing both the temporal and spectral representations allows the model to leverage complementary information from both domains, enhancing its ability to detect anomalies and infer causal relationships.

\textbf{Coefficient Projection}

\textbf{Projection.}
\begin{equation}
\mathbf{C}_{\text{time}} = \text{Linear}(\tilde{\mathbf{H}}^\text{time})
\end{equation}
This converts fused features into coefficient matrices. Specifcally, the coefficients represent variable-to-variable dependencies across lags.
This helps identify causal influences between variables (i.e., sensors or metrics such as how cpu usage affects memory usage over time).

\textbf{Lagged Prediction.}
\begin{equation}
\hat{\mathbf{x}}_\text{time} = \sum_{k=1}^K \mathbf{C}_{\text{time}} \, \mathbf{x}_{t-k}
\end{equation}
This predicts the next value using past windows. This approach captures autoregressive relationships, allowing the model to forecast future observations based on learned dependencies.

\textbf{Combination and Residual.}
\begin{equation}
\mathbf{z}_t = \mathbf{x}_t - \hat{\mathbf{x}}_t
\end{equation}
This computes the deviation from prediction. This computed z helps isolate exogenous factors not explained by past values. 
Subsecuntly, these exogenous variables are used by the decoder to reconstruct the original observations.

\subsubsection{Decoder Equations}

\textbf{Temporal Attention on Exogenous Inputs.}
\begin{equation}
\mathbf{H}^\text{temp}_t = \text{TemporalAttn}(\mathbf{H}^\text{enc}_{t-K+1:t})
\end{equation}
This aggregates information across the window. By attending to the sequence of inferred exogenous variables, the model captures temporal dependencies that are essential for accurate reconstruction of the original observations.

\textbf{Reconstruction.}
\begin{equation}
\hat{\mathbf{x}}_t = f_\text{out}(\mathbf{H}^\text{temp}_t)
\end{equation}
This produces the reconstructed output. The function $f_\text{out}$ maps the aggregated exogenous information back to the observation space, enabling the model to reconstruct the original multivariate time series.

\textbf{Low-Rank Coefficients.}
\begin{equation}
\mathbf{C}_t = \mathbf{U} \mathbf{V}^\top
\end{equation}
This builds a low-rank interaction matrix. Specifcally, the low-rank structure encourages simpler, more interpretable relationships between exogenous variables and observations.

\subsection{Training Objectives}

\textbf{Reconstruction Loss.}
\begin{equation}
\mathcal{L}_\text{recon} = \sum_{t} \|\hat{\mathbf{x}}_t - \mathbf{x}_t\|_2^2
\end{equation}
This penalizes reconstruction errors. For instance, minimizing this loss ensures that the model accurately captures the underlying data distribution, which is crucial for effective root cause analysis.

\textbf{Sparsity.}
\begin{equation}
\mathcal{L}_\text{sparse} = 
\lambda_\text{enc} R(\boldsymbol{\Omega}_t)
+ \lambda_\text{dec} (R(\bar{\boldsymbol{\Omega}}_t) + R(\bar{\boldsymbol{\Omega}}'_t))
\end{equation}
This encourages sparse coefficients. Specifcally, this promotes simpler causal structures by penalizing unnecessary connections between variables, making it easier to identify key root causes.

\textbf{Smoothness.}
\begin{equation}
\mathcal{L}_\text{smooth} =
\gamma_\text{enc} S(\boldsymbol{\Omega}_{t+1},\boldsymbol{\Omega}_t)
+ \gamma_\text{dec}(S(\bar{\boldsymbol{\Omega}}_{t+1},\bar{\boldsymbol{\Omega}}_t)
+ S(\bar{\boldsymbol{\Omega}}'_{t+1},\bar{\boldsymbol{\Omega}}'_t))
\end{equation}
This encourages coefficient stability across time. This loss ensures that the inferred relationships do not fluctuate wildly between consecutive time steps, which is important for maintaining consistent causal interpretations over time.

\textbf{KL Term.}
\begin{equation}
\mathcal{L}_\text{KL} = 
\frac{1}{2} \left(\mathrm{tr}(\Sigma_t) + \mu_t^\top \mu_t - d - \log \det \Sigma_t \right)
\end{equation}
This regularizes the latent space. By constraining the distribution of latent exogenous variables, this loss helps prevent overfitting and encourages the model to learn meaningful representations that generalize well to unseen data.

\textbf{Total Loss.}
\begin{equation}
\mathcal{L}_\text{total}
= \mathcal{L}_\text{recon}
+ \mathcal{L}_\text{sparse}
+ \mathcal{L}_\text{smooth}
+ \mathcal{L}_\text{KL}
\end{equation}
This is the final training objective.

\subsection{Root Cause Localization}

\begin{equation}
z_{t^*}^{(j)} =
\frac{z_{t^*}^{(j)} - \mu^{(j)}}{\sigma^{(j)}}
\end{equation}
This standardizes the exogenous variables for anomaly scoring. This approach highlights variables that deviate significantly from their normal behavior, aiding in the identification of potential root causes.


\subsection{Justification of Architectural Choices.}
Each module in Fig.~\ref{fig:SpectoGraphNet} is introduced to align the model’s computations with the underlying Granger-causal design. 

\textbf{Motivation}
Rootcause analysis in multivariate time series requires capturing complex interactions among variables over time. The architectural choices in CrGSTA are motivated by the need to effectively model these interactions while ensuring interpretability and scalability.
While prior works have explored interpetability using Granger Causality \cite{GVAR, 285-encoder-decoder}, their architectural choice lack the scalability of modeling long-range dependencies and the ability to capture both time and frequency domain information.
Specifcally, both these prior works rely on separate MLP per lag, while this allows for the interpretability of the learned coefficients, it easily becomes intractable when the number of lags increases.

\textbf{Graph Stduture.}
The graph structure captures variable interactions, essential for modeling causal relationships.
This was motivated by prior work demonstrating the effectiveness of graph-based methods for multivariate time series analysis~\cite{263-complexJournal,270-MSTGAD}.
This desgin choice allows for a better representation of the dependencies among variables, which is crucial for accurate root cause identification.

\textbf{Frequency Domain.}
Incorporating frequency-domain information enables the model to capture periodic patterns and anomalies that may not be evident in the time domain alone.
This dual-domain approach enhances the model's ability to detect anomalies and infer causal relationships, as certain anomalies may manifest more clearly in the spectral representation.
This was inspired by recent success of prior works on frequency-based time series modeling~\cite{276-Fits,280-FreqTimeLoss}.

\textbf{Spatial and Temporal Attention.}
The spatial attention mechanism allows the model to focus on the most relevant variables at each time step, while the temporal attention captures dependencies across time. 
This desgin choice allows the model to effectively learn complex interactions in both space and time, which is essential for accurate root cause analysis.
Additionally, it allows for a more parameter efficient representation compared to using separate attention mechanisms for each variable or time step while allowing for an interpretable attention weights that can be used for root cause identification.
This has been shown to be effective in prior works~\cite{270-MSTGAD}.

\textbf{Encoder-Decoder Structure.}
The encoder-decoder architecture separates the tasks of inferring exogenous variables and reconstructing observations.
This enables the model to learn a more structured representation of the data, facilitating the identification of root causes.
It builds on the success of prior works~\cite{285-encoder-decoder,263-complexJournal} that have demonstrated the effectiveness of this structure for
anomaly detection and root cause analysis.

\textbf{Cross-Attention Fusion.}
This innovative module allows the model to integrate information from both time and frequency domains.
It has been motivated by prior works~\cite{290-crosstimefreq-CrossFun,289-crosstimefreq-DeAnomaly} that have shown the benefits of combining temporal and spectral information for improved anomaly detection.

\begin{table}[H]
	\centering
	\renewcommand{\arraystretch}{1.25}
	\setlength{\tabcolsep}{3pt}
	\caption{CrGSTA Modules, Their Inspirations, and Motivations}
	\begin{tabular}{|p{3.8cm}|p{4.2cm}|p{6.2cm}|}
		\hline
		\textbf{Module} & \textbf{Inspiring Works} & \textbf{Why It Was Used} \\ \hline
		
		
		Graph Structure (Shared GNN)
		& \cite{263-complexJournal,270-MSTGAD}
		& Captures variable interactions and causal dependencies; provides a scalable structural prior replacing per-lag MLPs; improves interpretability and stability across domains. \\ \hline
		
		
		
		Frequency-Domain Module
		& \cite{276-Fits,280-FreqTimeLoss}
		& Extracts periodic and oscillatory patterns not visible in raw time series; improves anomaly detection sensitivity and complements time-domain reasoning. \\ \hline
		

		
		
		Spatial \& Temporal Attention
		& \cite{270-MSTGAD}
		& Learns variable relevance and long-range temporal structure; more parameter-efficient than per-variable attention; provides interpretable weights for RCA. \\ \hline
		
		
		Encoder–Decoder Structure
		& \cite{285-encoder-decoder,263-complexJournal}
		& Separates exogenous-variable inference from reconstruction; produces more structured latent representations and improves causal interpretability during anomalies. \\ \hline


		Cross-Attention Fusion
		& \cite{290-crosstimefreq-CrossFun,289-crosstimefreq-DeAnomaly}
		& Enables bidirectional fusion between temporal and spectral representations; captures anomalies that manifest differently across domains; enhances robustness. \\ \hline
	\end{tabular}
	\label{tab:module_inspiration}
\end{table}




%Freq from \cite{276-Fits}, \cite{280-FreqTimeLoss}
%Graph architecture \cite{263-complexJournal} \cite{270-MSTGAD}
%Encoder-decoder structure \cite{285-encoder-decoder}\cite{263-complexJournal}
%Temporal and spatial attention \cite{270-MSTGAD}
%Cross Time Freq \cite{290-crosstimefreq-CrossFun}, \cite{289-crosstimefreq-DeAnomaly}



\subsection{Evaluation Datasets and Metrics}
\subsubsection{Dataset}
\label{appendix:datasets}
\begin{table}[h]
	\centering
	\caption{Statistics of datasets.}
	\label{tab:datasets}
	\resizebox{\columnwidth}{!}{%
		\small
		\begin{tabular}{l c c c c }
			\toprule
			Dataset & Training Steps & Test Sequences ($|X|$) & Avg. Length ($T$) & Avg. Root Vars  \\
			\midrule
			\multicolumn{5}{|l|}{\cellcolor{gray!90} \textbf{Synthetic Datasets}} \\ \hline
			Nonlinear (20)  \cite{285-marcinkevics-lotka} & 5,000 & 100 & 500 & 5.25  \\
			Lotka–Volterra (40)  \cite{285-marcinkevics-lotka} & 40,000 & 100 & 2,000 & 30.75 \\
			\midrule
			\multicolumn{5}{|l|}{\cellcolor{gray!90} \textbf{Real-World Datasets}} \\ \hline
			SWaT (51) \cite{295-mathur2016-swat} & 49,500 & 20 & 51 & 13.35  \\
			MSDS (10) \cite{285-nedelkoski2020-msds} & 29,268 & 4,255 & 21 & 3.05 \\
			\bottomrule
		\end{tabular}%
	}
\end{table}



\paragraph{Lotka--Volterra (Extended).}  
\label{appendix:lotka}
Extending the work of Marcinkevičs \& Vogt~\cite{285-marcinkevics-lotka} and its implementation in~\cite{285-encoder-decoder}, we introduce additional nonlinearities, stochastic variability, and more realistic adversarial perturbations. Instead of the original formulation
\begin{align}
	\frac{dx^{(i)}}{dt} &= \alpha x^{(i)} - \beta \!\!\sum_{j \in Pa(x^{(i)})} y^{(j)} - \eta \big(x^{(i)}\big)^2, \\
	\frac{dy^{(j)}}{dt} &= \delta y^{(j)} \!\!\sum_{k \in Pa(y^{(j)})} x^{(k)} - \rho y^{(j)}, \\
	x^{(i)}_t &= x^{(i)}_t + 10\,\epsilon^{(i)}_t, \quad
	y^{(j)}_t = y^{(j)}_t + 10\,\epsilon^{(j)}_t, \quad 1 \leq i,j \leq p,
\end{align}
we build the extended version as
\begin{align}
	\frac{dx^{(i)}}{dt} &= \alpha x^{(i)} - \beta \!\!\sum_{j \in Pa(x^{(i)})} y^{(j)} - \eta \big(x^{(i)}\big)^2 + \cos\!\big(x^{(i)}\!+\!1\big) + 0.5 \sin\!\big(x^{(i)}\big) + \sigma \mathcal{N}(0,1), \\
	\frac{dy^{(j)}}{dt} &= \delta y^{(j)} \!\!\sum_{k \in Pa(y^{(j)})} x^{(k)} - \rho y^{(j)} + \cos\!\big(y^{(j)}\!+\!1\big) + 0.5 \sin\!\big(y^{(j)}\big) + \sigma \mathcal{N}(0,1), \\
	x^{(i)}_t &= x^{(i)}_t + 2\,\epsilon^{(i)}_t, \quad
	y^{(j)}_t = y^{(j)}_t + 2\,\epsilon^{(j)}_t, \quad 1 \leq i,j \leq p.
\end{align}

Here, $x^{(i)}$ and $y^{(j)}$ denote prey and predator populations, respectively; $\alpha, \beta, \eta, \delta, \rho$ are interaction parameters; $\sigma$ introduces stochastic fluctuations; and $\epsilon^{(\cdot)}_t$ represents adversarial perturbations. By replacing the anomaly multiplier of $10$ with $2$ and enriching the dynamics with sinusoidal and noise terms, the anomalies become more subtle and thus better reflect realistic system behavior.
Adding the $\cos$ and $\sin$ terms introduces richer nonlinear interactions, which better capture oscillatory and complex temporal behaviors often observed in ecological or real-world systems. These nonlinear contributions, combined with stochastic fluctuations, allow the model to exhibit more diverse dynamics, including variable growth rates, oscillations, and subtle chaotic effects. This makes the resulting datasets more challenging for anomaly detection and causal inference tasks, providing a closer approximation to realistic scenarios than the original Lotka--Volterra formulation.



\paragraph{Non--Linear (Extended).}  
\label{appendix:nonlinear-ar}

Extending standard synthetic autoregressive formulations and its implementation in~\cite{285-encoder-decoder}, we construct a significantly richer nonlinear generator that incorporates higher-order temporal dependencies, expressive nonlinear interactions, correlated stochastic noise, and a causal anomaly mechanism.  
Whereas the baseline model follows a simple linear recurrence,
\begin{align}
    x^{(i)}_t &= \sum_{l=1}^{L} A^{(l)}_{i:}\, x_{t-l} + \epsilon^{(i)}_t ,
\end{align}
our extended formulation introduces nonlinearity, lag-specific mixing, and structured variability:
\begin{align}
    x^{(i)}_t &=
    \sum_{l=1}^{5} A^{(l)}_{i:}
    \Big(
        \sin\!\big(x_{t-l} + 0.5\big)
        + \log\!\big(1 + |x_{t-l}|\big)
    \Big)
    + \epsilon^{(i)}_t .
\end{align}

Here each $A^{(l)}$ is obtained by scaling the underlying causal adjacency matrix with lag-dependent coefficients, enabling distinct temporal effects across the previous five time steps.  
The combination of $\sin(\cdot)$ and $\log(1 + |\cdot|)$ introduces oscillatory, amplitude-dependent, and mildly chaotic behavior, substantially increasing the complexity of the normal data compared to classical linear autoregressive processes.

We also introduce a causal anomaly mechanism that allows perturbations to persist and propagate through the system.  
For non-causal anomalies, deviations are added directly and instantaneously to the noise:
\begin{align}
    \epsilon^{(i)}_t \leftarrow \epsilon^{(i)}_t + a^{(i)}, 
    \qquad t \in \mathcal{T}_{\mathrm{anom}}.
\end{align}

To model anomalies that spread through the nonlinear temporal dynamics, we introduce a latent anomaly effect $z_t$ with exponential decay:
\begin{align}
    z_t &= 0.95\, z_{t-1} + a, 
    && t \in \mathcal{T}_{\mathrm{anom}}, \\
    z_t &= 0.95\, z_{t-1},
    && t \notin \mathcal{T}_{\mathrm{anom}}, \\
    \epsilon_t &\leftarrow \epsilon_t + z_t.
\end{align}

Injecting the perturbation into the noise---rather than directly modifying the state---forces the anomaly to propagate through the nonlinear transformation and multi-lag mixing structure, producing cascading effects that resemble fault propagation in realistic systems.



\subsubsection{Evaluation Metrics}
\label{appendix:metrics}

\paragraph{Recall at Top-$k$ (AC@$k$).}  
Following prior work~\cite{286-Ikram2022-RCD,285-li2022-recall}, we evaluate root cause identification using the \emph{recall at top-$k$} metric, denoted $\text{AC@}k$. This metric measures the likelihood that the true root causes appear within the top-$k$ ranked variables for each anomalous sequence.  

Formally, let $X \in \mathcal{X}$ denote an anomalous sequence, $R_X[k]$ the top-$k$ ranked variables produced by the model, and $V^{(\text{RC})}_X$ the ground-truth root cause set. Then,  

\begin{equation}
	\text{AC@}k =
	\frac{1}{|\mathcal{X}|} \sum_{X \in \mathcal{X}}
	\frac{\left| V^{(\text{RC})}_X \cap \{R_X[1], \ldots, R_X[k]\}\right|}
	{\min(k, |V^{(\text{RC})}_X|)}.
\end{equation}

This definition ensures normalization when multiple root causes exist, by dividing by $\min(k, |V^{(\text{RC})}_X|)$.  

\paragraph{Average Recall (Avg@$k$).}  
To summarize overall performance across different cutoffs, we also report the averaged metric:  
\begin{equation}
	\text{Avg@}k = \frac{1}{k} \sum_{i=1}^{k} \text{AC@}i.
\end{equation}

This provides a more comprehensive measure than a single cutoff.  

\paragraph{Multiple Interventions.}  
When a sequence contains multiple exogenous interventions, we treat it as a single root cause sequence, following the \emph{point-adjust evaluation} protocol~\cite{288-pointwise,290-pointwise}. This is consistent with the dominant evaluation setup for multivariate time series anomaly detection and root cause analysis.  

\paragraph{Model Efficiency.}  
In addition to accuracy metrics, we report the number of trainable parameters. This is particularly relevant for encoder–decoder architectures, where performance improvements may arise from increased capacity rather than architectural design. Reporting parameter counts allows us to assess the trade-off between accuracy and efficiency.  


\subsection{Implementation Details}
\label{appendix:implementation}
In this section, we summarize the key configurations used in our experiments (Tables~\ref{tab:swat_configs}, \ref{tab:lotka_configs}, and \ref{tab:nonlinear_configs} and \ref{tab:msds_configs}); full details are available in our released code. For AERCA, we adopt the original implementation~\cite{285-encoder-decoder} with its reported hyperparameters. For our CrGSTA model, we set the spatial–temporal attention dimension to 64 on Lotka–Volterra and 256 on SWaT, with 2 attention heads in both cases, we then use the same dimensions for other attention based baselines for a fair comparison. 
This approach is followed for Nonlinear and MSDS (albeit with different attention dimensions due to dataset size). For RQ3 ablations, we reduced the number of heads to isolate the impact of architectural choices. The decoder employs a lightweight self-attention layer with 64 hidden dimensions and 2 heads (32 for Lotka-Volterra). All models are trained with Adam (learning rate $10^{-4}$).

These parameter choices were informed by preliminary exploration and prior work, striking a balance between model expressiveness and computational efficiency. Rather than maximizing raw accuracy via larger dimensions or more heads, we deliberately used moderate settings to better highlight the architectural contributions of CrGSTA. Each experiment was repeated with multiple random seeds, and we report mean and standard deviation in the appendix for robustness.
We further mention the motivations behind certain hyperparameter choices below after the tables.

\begin{table}[H]
	\footnotesize
	\centering
	\renewcommand{\arraystretch}{1.25}
	\setlength{\tabcolsep}{5pt}
	\caption{Experiment Configurations for Lotka--Volterra Benchmark}
	\begin{tabular}{|p{2cm}|p{1.7cm}|p{1.7cm}|p{1.7cm}|p{2cm}|p{2cm}|}
		\hline
		\textbf{Key Parameter} & \textbf{FEDformer ¶} & \textbf{iTransformer ¶} & \textbf{CuasalRCA†} & \begin{tabular}{c}
\textbf{AERCA*} \\
\textbf{GVAR**} 
\end{tabular} & \textbf{CrGSTA} \\ \hline
		Learning Rate & 1e-4 & 1e-4 & 1e-4 & 1e-4 & 1e-4 \\ \hline
		Attention Dim & 64 & 64 & -- & -- &(spatial 64) (temporal 64) (decoder 50)\\ \hline
		Attention Heads & 2 & 2 & -- & -- &(spatial 2) (temporal 2) (decoder 2) \\ \hline
		MLP layers (dim) & -- & -- & 256 & 2 layers (50 nodes) per lag & -- \\ \hline
		Num Variables & 40 & 40 & 40 &20 & 40 \\ \hline
		Epochs & 100 & 100 & 100 & 5000 (with early stopping) & 100 \\ \hline
	\end{tabular}
	\label{tab:lotka_configs}
\end{table}

\begin{table}[H]
	\footnotesize
	\centering
	\renewcommand{\arraystretch}{1.25}
	\setlength{\tabcolsep}{5pt}
	\caption{Experiment Configurations for SWaT Benchmark}
	\begin{tabular}{|p{2cm}|p{1.7cm}|p{1.7cm}|p{1.7cm}|p{2cm}|p{2cm}|}
		\hline
		\textbf{Key Parameter} & \textbf{FEDformer ¶} & \textbf{iTransformer ¶} & \textbf{CuasalRCA†} & \begin{tabular}{c}
\textbf{AERCA*} \\
\textbf{GVAR**} 
\end{tabular} & \textbf{CrGSTA} \\ \hline
		Learning Rate & 1e-4 & 1e-4 & 1e-4 & 1e-6 & 1e-4 \\ \hline
		Attention Dim & 256 & 256 & -- & --& (spatial 256) (temporal 256) (decoder 64) \\ \hline
		Attention Heads & 2 & 2 & -- & --& (spatial 2) (temporal 2) (decoder 2) \\ \hline
		MLP layers (dim) & -- & -- & 256 & 8 layers (1000 nodes) per lag & -- \\ \hline
		Epochs & 1000 & 1000   & 1000 & 5000 (with early stopping) & 1000 \\ \hline
	\end{tabular}
	\label{tab:swat_configs}
\end{table}


\begin{table}[H]
	\footnotesize
	\centering
	\renewcommand{\arraystretch}{1.25}
	\setlength{\tabcolsep}{5pt}
	\caption{Experiment Configurations for NonLinear Benchmark}
	\begin{tabular}{|p{2cm}|p{1.7cm}|p{1.7cm}|p{1.7cm}|p{2cm}|p{2cm}|}
		\hline
		\textbf{Key Parameter} & \textbf{FEDformer ¶} & \textbf{iTransformer ¶} & \textbf{CuasalRCA†} & \begin{tabular}{c}
\textbf{AERCA*} \\
\textbf{GVAR**} 
\end{tabular} & \textbf{CrGSTA} \\ \hline
		Learning Rate & 1e-4 & 1e-4 & 1e-4 & 1e-4 & 1e-4 \\ \hline
		Attention Dim & 64 & 64 & -- & -- &(spatial 64) (temporal 64) (decoder 50)\\ \hline
		Attention Heads & 2 & 2 & -- & -- &(spatial 2) (temporal 2) (decoder 2) \\ \hline
		MLP layers (dim) & -- & -- & 256 & 8 layers (50 nodes) per lag & -- \\ \hline
		Num Variables & 20 & 20 & 20 &20 & 20 \\ \hline
		Epochs & 100 & 100 & 100 & 100 & 100 \\ \hline
	\end{tabular}
	\label{tab:nonlinear_configs}
\end{table}


\begin{table}[H]
	\footnotesize
	\centering
	\renewcommand{\arraystretch}{1.25}
	\setlength{\tabcolsep}{5pt}
	\caption{Experiment Configurations for MSDS Benchmark}
	\begin{tabular}{|p{2cm}|p{1.7cm}|p{1.7cm}|p{1.7cm}|p{2cm}|p{2cm}|}
		\hline
		\textbf{Key Parameter} & \textbf{FEDformer ¶} & \textbf{iTransformer ¶} & \textbf{CuasalRCA†} & \begin{tabular}{c}
\textbf{AERCA*} \\
\textbf{GVAR**} 
\end{tabular} & \textbf{CrGSTA} \\ \hline
		Learning Rate & 1e-4 & 1e-4 & 1e-4 & 1e-6 & 1e-4 \\ \hline
		Attention Dim & 16 & 16 & -- & -- &(spatial 16) (temporal 16) (decoder 50)\\ \hline
		Attention Heads & 2 & 2 & -- & -- &(spatial 2) (temporal 2) (decoder 2) \\ \hline
		MLP layers (dim) & -- & -- & 256 & 4 layers (1000 nodes) per lag & -- \\ \hline
		Num Variables & 10 & 10 & 10 &10 & 10 \\ \hline
		Epochs & 1000 & 1000 & 1000 & 5000 (with early stopping) & 1000 \\ \hline
	\end{tabular}
	\label{tab:msds_configs}
\end{table}

\subsubsection{Motivations for Specific Parameter Choices}
\textbf{FEDformer ¶, iTransformer ¶}:
For FEDformer and iTransformer, for fair comparison, we used the same attention dimension and number of heads as CrGSTA on each dataset.
This allows for a more direct comparison of the architectural choices rather than differences in model capacity.


\textbf{CausalRCA†}:
CausalRCA architecture is relatively simple compared to AERCA and CrGSTA.
It is composed of two linear layers with a ReLU activation in between. 
So for fair comparison, we increased the hidden dimension to 256, to increase the model capacity, to be competitive in performance with other models.
This desgin choice allowed CausalRCA to be competitive in performance especially for synthetic datasets, such as Lotka-Volterra and Non-Linear datasets.


\textbf{AERCA*}:
AERCA parameters are adopted from the original implementation~\cite{285-encoder-decoder}.
We note that AERCA uses a separate MLP per lag to model temporal dependencies, which limits scalability to longer windows.
This desgin choice, which has been inherited from GVAR~\cite{GVAR}, results in a linear increase in the number of parameters as the window size increases.
This has been the motivation for our CrGSTA model to use a shared graph structure across time lags, which allows for a more parameter efficient representation. 

\textbf{GVAR**}:
GVAR architecture \cite{GVAR} is an encoder that uses a separate MLP per lag to model temporal dependencies.
AERCA builds on this by adding two decoders built using the same per-lag MLP structure. Moreover, AERCA added 
KL regularization, decoder smoothness, and decoder sparsity losses to the training objective.
For the reconstruction loss, GVAR reconstructs the whole time series window, while AERCA reconstructs the shifted window due to its encoder-decoder structure.
To ensure a fair comparison, we implemented GVAR version using the encoder architecture as AERCA, while removing the decoder modules and their associated losses from the training objective including the KL regularization, and used for reconstruction the whole time series window as in the original GVAR.






\subsection{Full Results}
\label{Appendix:full_results}
In this section, we provide the set of full tables and figures for the experiments in RQ1, RQ2 and RQ3 from the main paper. Moreover, we include additional analysis and discussion of the results.

\subsubsection{RQ1 (temporal dimension) - Full Tables}
\label{appendix:RQ1-full-tables}
In this experiment, we investigate the impact of varying the temporal window size on root cause identification performance. We evaluate a range of window sizes from 1 to 12 time steps, assessing how this parameter influences the model's ability to accurately identify root causes in both the Lotka–Volterra, Non-Linear  SWaT and MSDS datasets.


\paragraph{Parameter Scaling.}
Figure~\ref{fig:RQ1-params} illustrates how the number of trainable parameters scales with increasing temporal window sizes for all the different datasets. Notably, CrGSTA maintains a relatively stable parameter count across window sizes, demonstrating its efficiency in handling longer temporal contexts without a significant increase in model complexity. In contrast, GVAR and AERCA exhibit a linear growth in parameters as the window size increases, which can lead to scalability challenges for larger windows. This efficiency of CrGSTA is particularly advantageous for practical applications where computational resources may be limited.


%\textbf{Statistical Methods.} Epsilon and RCD remain unaffected by window size, as they do not incorporate temporal information.
%\\
%\textbf{Generic Time Series Models.} iTransformer and FEDformer achieve slight improvements as windows increase, confirming that temporal context aids root cause identification. However, their gains remain marginal compared to causal models.
%\\
%\textbf{Causal Inference Models.} AERCA and CrGSTA benefit substantially from larger windows, confirming that causal inference frameworks exploit extended temporal dependencies more effectively. Importantly, while AERCA achieves strong AC@1 scores on Lotka–Volterra, CrGSTA consistently delivers the best Avg@10 performance across window sizes and datasets. This is particularly significant, since Avg@10 better reflects a model’s practical utility by balancing precision at multiple ranks rather than focusing only on the very top prediction.
%\\
%\textbf{AERCA vs. CrGSTA.} Both models scale with window size, but CrGSTA’s parameter efficiency and superior Avg@10 results highlight its advantage. AERCA, despite linearly increasing parameters and achieving sharp AC@1 peaks, is constrained by memory at larger windows and fails to surpass CrGSTA in Avg@10. Notably, for Lotka–Volterra, AERCA’s best Avg@10 (0.803 at window 5) falls below CrGSTA’s peak (0.782 at window 7) once parameter cost is considered, since CrGSTA maintains high performance with only 1.0M parameters while AERCA requires more than triple the capacity. This demonstrates that CrGSTA achieves a better balance of performance and efficiency, making it more robust for practical RCA scenarios.
%
%\textbf{Summary.} Larger temporal windows enhance accuracy across methods, but causal inference models benefit the most. While AERCA excels in AC@1 at specific windows, CrGSTA dominates in Avg@10, the more reliable metric for practical RCA, while requiring far fewer parameters. These results establish CrGSTA as the most effective and efficient model for leveraging temporal context in multivariate root cause analysis.


\begin{figure}[htbp]
	\centering
	% Subfigure (a)
	\begin{subfigure}[b]{0.45\textwidth}
		\centering
		\includegraphics[width=\textwidth]{Scripts/Data/CrGSTA/params_vs_windows_Lotka.pdf}
		\caption{Lotka Volterra Parameters}
	\end{subfigure}
	\hfill
	% Subfigure (b)
	\begin{subfigure}[b]{0.45\textwidth}
		\centering
		\includegraphics[width=\textwidth]{Scripts/Data/CrGSTA/params_vs_windows_swat.pdf}
		\caption{SWAT Parameters}
	\end{subfigure}
	\hfill
	\begin{subfigure}[b]{0.45\textwidth}
		\centering
		\includegraphics[width=\textwidth]{Scripts/Data/CrGSTA/params_vs_windows_nonlinear.pdf}
		\caption{Non-Linear Parameters}
	\end{subfigure}
	\hfill
	% Subfigure (b)
	\begin{subfigure}[b]{0.45\textwidth}
		\centering
		\includegraphics[width=\textwidth]{Scripts/Data/CrGSTA/params_vs_windows_msds.pdf}
		\caption{MSDS Parameters}
	\end{subfigure}
	
	\caption{Parameter scaling for Lotka Volterra (left) and SWAT (right) for temporal scaling.}
	\label{fig:RQ1-params}
\end{figure}

\paragraph{Full Results Tables}
\label{appendix:RQ1-full-tables-results}
In this section, we present the complete results for the temporal window size experiments on the different datasets. The tables below summarize the performance of various models across a range of window sizes, providing detailed insights into how temporal context influences root cause identification accuracy.
Specifcally, we report the AC@1, AC@3, AC@5, AC@10, and Avg@10 metrics for each model and window size configuration. Moreover, we include the number of trainable parameters for each model to facilitate a comprehensive comparison of performance relative to model complexity.
Due to the space limitations in the main paper, we inclue the detailed analysis of both Non-Linear and MSDS datasets here, while the Lotka Volterra results and MSDS are presented in the main paper.





\begin{table}[H]
\begin{tabular}{llllllll}
	\toprule
	scheme & Params & window size & AC@1 & AC@3 & AC@5 & AC@10 & Avg@10 \\
	\midrule
	
	\midrule
	\rowcolor{gray!20} \multicolumn{8}{c}{LOTKA VOLTERRA} \\
	iTransformer & 0.052M & 10 & 0.060\tiny{±0.010} & 0.089\tiny{±0.004} & 0.120\tiny{±0.005} & 0.234\tiny{±0.006} & 0.139\tiny{±0.002} \\
	iTransformer & 0.052M & 7 & 0.090\tiny{±0.017} & 0.070\tiny{±0.012} & 0.101\tiny{±0.010} & 0.222\tiny{±0.018} & 0.128\tiny{±0.008} \\
	FEDformer & 0.2M & 12 & 0.100\tiny{±0.030} & 0.099\tiny{±0.004} & 0.133\tiny{±0.008} & 0.268\tiny{±0.021} & 0.162\tiny{±0.012} \\    
	FEDformer & 0.1M & 1 & 0.103\tiny{±0.015} & 0.102\tiny{±0.008} & 0.115\tiny{±0.010} & 0.233\tiny{±0.007} & 0.143\tiny{±0.003} \\     
	iTransformer & 0.051M & 5 & 0.107\tiny{±0.032} & 0.100\tiny{±0.012} & 0.109\tiny{±0.010} & 0.234\tiny{±0.014} & 0.146\tiny{±0.008} \\
	iTransformer & 0.052M & 12 & 0.107\tiny{±0.032} & 0.090\tiny{±0.006} & 0.122\tiny{±0.007} & 0.219\tiny{±0.005} & 0.140\tiny{±0.002} \\
	FEDformer & 0.1M & 7 & 0.120\tiny{±0.046} & 0.106\tiny{±0.022} & 0.129\tiny{±0.016} & 0.278\tiny{±0.011} & 0.168\tiny{±0.013} \\     
	RCD & 0.000M & 1 & 0.120\tiny{±0.000} & 0.150\tiny{±0.000} & 0.157\tiny{±0.000} & 0.267\tiny{±0.000} & 0.185\tiny{±0.000} \\
	RCD & 0.000M & 5 & 0.120\tiny{±0.000} & 0.150\tiny{±0.000} & 0.157\tiny{±0.000} & 0.267\tiny{±0.000} & 0.185\tiny{±0.000} \\
	RCD & 0.000M & 7 & 0.120\tiny{±0.000} & 0.150\tiny{±0.000} & 0.157\tiny{±0.000} & 0.267\tiny{±0.000} & 0.185\tiny{±0.000} \\
	RCD & 0.000M & 10 & 0.120\tiny{±0.000} & 0.150\tiny{±0.000} & 0.157\tiny{±0.000} & 0.267\tiny{±0.000} & 0.185\tiny{±0.000} \\        
	RCD & 0.000M & 12 & 0.120\tiny{±0.000} & 0.150\tiny{±0.000} & 0.157\tiny{±0.000} & 0.267\tiny{±0.000} & 0.185\tiny{±0.000} \\        
	iTransformer & 0.051M & 1 & 0.127\tiny{±0.015} & 0.112\tiny{±0.013} & 0.139\tiny{±0.005} & 0.249\tiny{±0.016} & 0.166\tiny{±0.012} \\
	FEDformer & 0.2M & 10 & 0.137\tiny{±0.055} & 0.111\tiny{±0.023} & 0.132\tiny{±0.014} & 0.271\tiny{±0.011} & 0.168\tiny{±0.018} \\    
	FEDformer & 0.1M & 5 & 0.140\tiny{±0.036} & 0.120\tiny{±0.017} & 0.142\tiny{±0.013} & 0.275\tiny{±0.028} & 0.175\tiny{±0.006} \\     
	Epsilon & 0.000M & 1 & 0.150\tiny{±0.000} & 0.113\tiny{±0.000} & 0.145\tiny{±0.000} & 0.243\tiny{±0.000} & 0.167\tiny{±0.000} \\     
	Epsilon & 0.000M & 5 & 0.150\tiny{±0.000} & 0.113\tiny{±0.000} & 0.145\tiny{±0.000} & 0.243\tiny{±0.000} & 0.167\tiny{±0.000} \\     
	Epsilon & 0.000M & 7 & 0.150\tiny{±0.000} & 0.113\tiny{±0.000} & 0.145\tiny{±0.000} & 0.243\tiny{±0.000} & 0.167\tiny{±0.000} \\     
	Epsilon & 0.000M & 10 & 0.150\tiny{±0.000} & 0.113\tiny{±0.000} & 0.145\tiny{±0.000} & 0.243\tiny{±0.000} & 0.167\tiny{±0.000} \\    
	Epsilon & 0.000M & 12 & 0.150\tiny{±0.000} & 0.113\tiny{±0.000} & 0.145\tiny{±0.000} & 0.243\tiny{±0.000} & 0.167\tiny{±0.000} \\    
	GVAR & 1.0M & 12 & 0.421\tiny{±0.037} & 0.334\tiny{±0.016} & 0.362\tiny{±0.018} & 0.558\tiny{±0.022} & 0.426\tiny{±0.021} \\
	GVAR & 0.9M & 10 & 0.483\tiny{±0.045} & 0.366\tiny{±0.038} & 0.390\tiny{±0.026} & 0.586\tiny{±0.016} & 0.459\tiny{±0.024} \\
	GVAR & 0.6M & 7 & 0.560\tiny{±0.011} & 0.418\tiny{±0.006} & 0.436\tiny{±0.019} & 0.634\tiny{±0.012} & 0.510\tiny{±0.011} \\
	GVAR & 0.4M & 5 & 0.641\tiny{±0.016} & 0.495\tiny{±0.004} & 0.514\tiny{±0.009} & 0.704\tiny{±0.008} & 0.590\tiny{±0.007} \\
	AERCA & 0.3M & 1 & 0.740\tiny{±0.017} & 0.524\tiny{±0.015} & 0.488\tiny{±0.018} & 0.662\tiny{±0.003} & 0.584\tiny{±0.010} \\
	CrGSTA & 1.0M & 1 & 0.750\tiny{±0.026} & 0.520\tiny{±0.019} & 0.481\tiny{±0.023} & 0.648\tiny{±0.007} & 0.576\tiny{±0.014} \\        
	GVAR & 0.086M & 1 & 0.763\tiny{±0.016} & 0.547\tiny{±0.011} & 0.531\tiny{±0.009} & 0.705\tiny{±0.007} & 0.621\tiny{±0.008} \\        
	CrGSTA & 1.0M & 5 & 0.770\tiny{±0.030} & 0.524\tiny{±0.032} & 0.493\tiny{±0.010} & 0.658\tiny{±0.004} & 0.590\tiny{±0.012} \\        
	CrGSTA & 1.0M & 12 & 0.770\tiny{±0.046} & 0.513\tiny{±0.018} & 0.486\tiny{±0.012} & 0.661\tiny{±0.013} & 0.585\tiny{±0.017} \\       
	CrGSTA & 1.0M & 10 & 0.880\tiny{±0.028} & 0.663\tiny{±0.009} & 0.589\tiny{±0.014} & 0.748\tiny{±0.005} & 0.694\tiny{±0.003} \\       
	CrGSTA & 1.0M & 7 & 0.930\tiny{±0.028} & 0.753\tiny{±0.000} & 0.682\tiny{±0.011} & \textbf{0.845\tiny{±0.004}} & 0.782\tiny{±0.008} \\
	AERCA & 3.1M & 12 & 0.930\tiny{±0.014} & 0.703\tiny{±0.014} & 0.666\tiny{±0.004} & 0.805\tiny{±0.010} & 0.758\tiny{±0.003} \\        
	AERCA & 2.6M & 10 & 0.935\tiny{±0.007} & 0.735\tiny{±0.012} & 0.669\tiny{±0.022} & \underline{0.817\tiny{±0.006}} & 0.769\tiny{±0.007} \\
	causalrca & 0.004M & 1 & 0.963\tiny{±0.004} & 0.742\tiny{±0.011} & 0.642\tiny{±0.007} & 0.763\tiny{±0.002} & 0.745\tiny{±0.005} \\   
	causalrca & 0.004M & 5 & 0.963\tiny{±0.004} & 0.741\tiny{±0.011} & 0.642\tiny{±0.007} & 0.762\tiny{±0.003} & 0.745\tiny{±0.005} \\   
	causalrca & 0.004M & 7 & 0.963\tiny{±0.004} & 0.742\tiny{±0.011} & 0.641\tiny{±0.007} & 0.762\tiny{±0.003} & 0.745\tiny{±0.006} \\   
	causalrca & 0.004M & 10 & 0.963\tiny{±0.004} & 0.742\tiny{±0.011} & 0.641\tiny{±0.007} & 0.762\tiny{±0.002} & 0.745\tiny{±0.005} \\  
	causalrca & 0.004M & 12 & 0.963\tiny{±0.004} & 0.742\tiny{±0.011} & 0.641\tiny{±0.007} & 0.762\tiny{±0.003} & 0.745\tiny{±0.005} \\  
	AERCA & 1.8M & 7 & \underline{0.970\tiny{±0.026}} & \underline{0.764\tiny{±0.031}} & \underline{0.697\tiny{±0.023}} & 0.814\tiny{±0.026} & \underline{0.791\tiny{±0.017}} \\
	AERCA & 1.3M & 5 & \textbf{0.977\tiny{±0.006}} & \textbf{0.788\tiny{±0.007}} & \textbf{0.717\tiny{±0.010}} & 0.816\tiny{±0.008} & \textbf{0.803\tiny{±0.003}} \\
	\bottomrule
\end{tabular}
	\caption{RQ1 Lotka Windows}
	\label{table:RQ1_lotka}
\end{table}





\begin{table}[H]
\begin{tabular}{llllllll}
	\toprule
	scheme & Params & window size & AC@1 & AC@3 & AC@5 & AC@10 & Avg@10 \\
	\midrule
	
	\midrule
	\rowcolor{gray!20} \multicolumn{8}{c}{SWAT} \\
	GVAR & 116.0M & 12 & - & - & - & - & - \\
	AERCA & 144.9M & 5 & - & - & - & - & - \\
	AERCA & 202.9M & 7 & - & - & - & - & - \\
	AERCA & 289.9M & 10 & - & - & - & - & - \\
	AERCA & 347.9M & 12 & - & - & - & - & - \\
	Epsilon & 0.000M & 5 & 0.000\tiny{±0.000} & 0.100\tiny{±0.000} & 0.100\tiny{±0.000} & 0.300\tiny{±0.000} & 0.140\tiny{±0.000} \\
	Epsilon & 0.000M & 12 & 0.000\tiny{±0.000} & 0.025\tiny{±0.000} & 0.025\tiny{±0.000} & 0.275\tiny{±0.000} & 0.070\tiny{±0.000} \\
	RCD & 0.000M & 1 & 0.000\tiny{±0.000} & 0.000\tiny{±0.000} & 0.000\tiny{±0.000} & 0.300\tiny{±0.000} & 0.100\tiny{±0.000} \\    
	RCD & 0.000M & 5 & 0.000\tiny{±0.000} & 0.000\tiny{±0.000} & 0.000\tiny{±0.000} & 0.300\tiny{±0.000} & 0.100\tiny{±0.000} \\    
	RCD & 0.000M & 7 & 0.000\tiny{±0.000} & 0.000\tiny{±0.000} & 0.000\tiny{±0.000} & 0.300\tiny{±0.000} & 0.100\tiny{±0.000} \\    
	RCD & 0.000M & 10 & 0.000\tiny{±0.000} & 0.000\tiny{±0.000} & 0.000\tiny{±0.000} & 0.300\tiny{±0.000} & 0.100\tiny{±0.000} \\   
	RCD & 0.000M & 12 & 0.000\tiny{±0.000} & 0.000\tiny{±0.000} & 0.000\tiny{±0.000} & 0.300\tiny{±0.000} & 0.100\tiny{±0.000} \\   
	iTransformer & 0.8M & 10 & 0.031\tiny{±0.002} & 0.116\tiny{±0.008} & 0.215\tiny{±0.008} & 0.387\tiny{±0.014} & 0.208\tiny{±0.002} \\
	iTransformer & 0.8M & 7 & 0.043\tiny{±0.000} & 0.108\tiny{±0.009} & 0.170\tiny{±0.013} & 0.417\tiny{±0.015} & 0.206\tiny{±0.004} \\
	iTransformer & 0.8M & 12 & 0.044\tiny{±0.002} & 0.098\tiny{±0.007} & 0.215\tiny{±0.005} & 0.364\tiny{±0.006} & 0.203\tiny{±0.002} \\
	Epsilon & 0.000M & 7 & 0.050\tiny{±0.000} & 0.075\tiny{±0.000} & 0.075\tiny{±0.000} & 0.375\tiny{±0.000} & 0.110\tiny{±0.000} \\
	Epsilon & 0.000M & 10 & 0.050\tiny{±0.000} & 0.100\tiny{±0.000} & 0.100\tiny{±0.000} & 0.300\tiny{±0.000} & 0.142\tiny{±0.000} \\
	FEDformer & 2.4M & 12 & 0.054\tiny{±0.000} & 0.058\tiny{±0.000} & 0.109\tiny{±0.003} & 0.235\tiny{±0.040} & 0.124\tiny{±0.008} \\
	causalrca & 0.007M & 7 & 0.058\tiny{±0.029} & 0.084\tiny{±0.035} & 0.122\tiny{±0.031} & 0.261\tiny{±0.007} & 0.148\tiny{±0.022} \\
	FEDformer & 2.2M & 10 & 0.060\tiny{±0.000} & 0.061\tiny{±0.001} & 0.113\tiny{±0.000} & 0.278\tiny{±0.010} & 0.134\tiny{±0.003} \\
	FEDformer & 1.9M & 7 & 0.064\tiny{±0.000} & 0.068\tiny{±0.000} & 0.115\tiny{±0.006} & 0.292\tiny{±0.029} & 0.142\tiny{±0.003} \\
	causalrca & 0.007M & 5 & 0.069\tiny{±0.037} & 0.109\tiny{±0.040} & 0.127\tiny{±0.038} & 0.357\tiny{±0.029} & 0.178\tiny{±0.031} \\
	FEDformer & 1.9M & 5 & 0.070\tiny{±0.000} & 0.083\tiny{±0.004} & 0.133\tiny{±0.004} & 0.297\tiny{±0.028} & 0.152\tiny{±0.005} \\
	iTransformer & 0.8M & 5 & 0.073\tiny{±0.010} & 0.143\tiny{±0.004} & 0.250\tiny{±0.012} & 0.498\tiny{±0.013} & 0.267\tiny{±0.004} \\
	Epsilon & 0.000M & 1 & 0.100\tiny{±0.000} & 0.150\tiny{±0.000} & 0.150\tiny{±0.000} & 0.350\tiny{±0.000} & 0.170\tiny{±0.000} \\
	causalrca & 0.007M & 1 & 0.117\tiny{±0.035} & 0.164\tiny{±0.036} & 0.197\tiny{±0.045} & 0.294\tiny{±0.027} & 0.214\tiny{±0.031} \\
	AERCA & 29.0M & 1 & 0.150\tiny{±0.045} & 0.250\tiny{±0.045} & 0.317\tiny{±0.026} & 0.342\tiny{±0.038} & 0.289\tiny{±0.004} \\   
	iTransformer & 0.8M & 1 & 0.150\tiny{±0.060} & 0.217\tiny{±0.067} & 0.279\tiny{±0.099} & 0.400\tiny{±0.117} & 0.285\tiny{±0.083} \\
	GVAR & 9.7M & 1 & 0.167\tiny{±0.021} & 0.282\tiny{±0.059} & 0.341\tiny{±0.054} & 0.475\tiny{±0.098} & 0.348\tiny{±0.052} \\     
	causalrca & 0.007M & 10 & 0.185\tiny{±0.017} & 0.239\tiny{±0.003} & 0.248\tiny{±0.014} & 0.351\tiny{±0.021} & 0.263\tiny{±0.011} \\
	FEDformer & 1.6M & 1 & 0.208\tiny{±0.019} & 0.325\tiny{±0.000} & 0.325\tiny{±0.000} & 0.498\tiny{±0.039} & 0.349\tiny{±0.008} \\
	causalrca & 0.007M & 12 & 0.209\tiny{±0.005} & 0.237\tiny{±0.000} & 0.242\tiny{±0.000} & 0.313\tiny{±0.011} & 0.251\tiny{±0.002} \\
	CrGSTA & 8.5M & 1 & 0.225\tiny{±0.104} & 0.275\tiny{±0.061} & 0.333\tiny{±0.041} & 0.417\tiny{±0.054} & 0.327\tiny{±0.045} \\   
	CrGSTA & 8.5M & 12 & 0.275\tiny{±0.028} & 0.369\tiny{±0.036} & 0.415\tiny{±0.052} & 0.469\tiny{±0.058} & 0.404\tiny{±0.046} \\  
	GVAR & 48.3M & 5 & 0.277\tiny{±0.024} & 0.388\tiny{±0.024} & 0.419\tiny{±0.039} & 0.521\tiny{±0.051} & 0.429\tiny{±0.026} \\    
	CrGSTA & 8.5M & 5 & 0.282\tiny{±0.056} & 0.361\tiny{±0.035} & 0.366\tiny{±0.035} & 0.412\tiny{±0.078} & 0.368\tiny{±0.042} \\   
	GVAR & 67.6M & 7 & 0.285\tiny{±0.020} & \underline{0.411\tiny{±0.028}} & \underline{0.458\tiny{±0.023}} & \underline{0.564\tiny{±0.038}} & \underline{0.462\tiny{±0.027}} \\
	CrGSTA & 8.5M & 10 & 0.305\tiny{±0.047} & 0.397\tiny{±0.065} & 0.428\tiny{±0.065} & 0.472\tiny{±0.056} & 0.418\tiny{±0.057} \\  
	CrGSTA & 8.5M & 7 & 0.308\tiny{±0.037} & 0.396\tiny{±0.034} & 0.433\tiny{±0.030} & 0.488\tiny{±0.054} & 0.426\tiny{±0.031} \\   
	GVAR & 96.6M & 10 & \textbf{0.339\tiny{±0.004}} & \textbf{0.462\tiny{±0.019}} & \textbf{0.502\tiny{±0.037}} & \textbf{0.592\tiny{±0.039}} & \textbf{0.502\tiny{±0.025}} \\
	\bottomrule
\end{tabular}
	\caption{RQ1 Swat Windows}
	\label{table:RQ1_swat}
\end{table}


\begin{table}[H]
\begin{tabular}{llllllll}
\toprule
scheme & Params & window size & AC@1 & AC@3 & AC@5 & AC@10 & Avg@10 \\
\midrule

\midrule
\rowcolor{gray!20} \multicolumn{8}{c}{NONLINEAR} \\
Epsilon & 0.000M & 1 & 0.180\tiny{±0.000} & 0.307\tiny{±0.000} & 0.341\tiny{±0.000} & 0.530\tiny{±0.000} & 0.359\tiny{±0.000} \\
Epsilon & 0.000M & 3 & 0.180\tiny{±0.000} & 0.307\tiny{±0.000} & 0.341\tiny{±0.000} & 0.530\tiny{±0.000} & 0.359\tiny{±0.000} \\
Epsilon & 0.000M & 5 & 0.180\tiny{±0.000} & 0.307\tiny{±0.000} & 0.341\tiny{±0.000} & 0.530\tiny{±0.000} & 0.359\tiny{±0.000} \\
Epsilon & 0.000M & 7 & 0.180\tiny{±0.000} & 0.307\tiny{±0.000} & 0.341\tiny{±0.000} & 0.530\tiny{±0.000} & 0.359\tiny{±0.000} \\
Epsilon & 0.000M & 10 & 0.180\tiny{±0.000} & 0.307\tiny{±0.000} & 0.341\tiny{±0.000} & 0.530\tiny{±0.000} & 0.359\tiny{±0.000} \\
FEDformer & 0.1M & 5 & 0.217\tiny{±0.018} & 0.262\tiny{±0.013} & 0.281\tiny{±0.010} & 0.429\tiny{±0.012} & 0.306\tiny{±0.009} \\
iTransformer & 0.051M & 5 & 0.225\tiny{±0.012} & 0.262\tiny{±0.006} & 0.304\tiny{±0.005} & 0.453\tiny{±0.006} & 0.322\tiny{±0.002} \\
FEDformer & 0.1M & 10 & 0.230\tiny{±0.031} & 0.255\tiny{±0.018} & 0.294\tiny{±0.016} & 0.480\tiny{±0.013} & 0.328\tiny{±0.011} \\
RCD & 0.000M & 1 & 0.230\tiny{±0.000} & 0.250\tiny{±0.000} & 0.286\tiny{±0.000} & 0.519\tiny{±0.000} & 0.337\tiny{±0.000} \\
RCD & 0.000M & 3 & 0.230\tiny{±0.000} & 0.250\tiny{±0.000} & 0.286\tiny{±0.000} & 0.519\tiny{±0.000} & 0.337\tiny{±0.000} \\
RCD & 0.000M & 5 & 0.230\tiny{±0.000} & 0.250\tiny{±0.000} & 0.286\tiny{±0.000} & 0.519\tiny{±0.000} & 0.337\tiny{±0.000} \\
RCD & 0.000M & 7 & 0.230\tiny{±0.000} & 0.250\tiny{±0.000} & 0.286\tiny{±0.000} & 0.519\tiny{±0.000} & 0.337\tiny{±0.000} \\
RCD & 0.000M & 10 & 0.230\tiny{±0.000} & 0.250\tiny{±0.000} & 0.286\tiny{±0.000} & 0.519\tiny{±0.000} & 0.337\tiny{±0.000} \\
FEDformer & 0.1M & 3 & 0.235\tiny{±0.013} & 0.312\tiny{±0.006} & 0.365\tiny{±0.005} & 0.536\tiny{±0.011} & 0.387\tiny{±0.005} \\
FEDformer & 0.1M & 7 & 0.250\tiny{±0.024} & 0.257\tiny{±0.016} & 0.292\tiny{±0.011} & 0.469\tiny{±0.015} & 0.324\tiny{±0.005} \\
iTransformer & 0.052M & 7 & 0.251\tiny{±0.026} & 0.245\tiny{±0.019} & 0.282\tiny{±0.019} & 0.463\tiny{±0.017} & 0.319\tiny{±0.014} \\
iTransformer & 0.051M & 1 & 0.253\tiny{±0.057} & 0.280\tiny{±0.039} & 0.326\tiny{±0.020} & 0.507\tiny{±0.028} & 0.357\tiny{±0.028} \\
iTransformer & 0.052M & 10 & 0.284\tiny{±0.028} & 0.277\tiny{±0.013} & 0.302\tiny{±0.013} & 0.462\tiny{±0.014} & 0.337\tiny{±0.008} \\
iTransformer & 0.051M & 3 & 0.307\tiny{±0.012} & 0.311\tiny{±0.006} & 0.357\tiny{±0.006} & 0.514\tiny{±0.004} & 0.383\tiny{±0.002} \\
FEDformer & 0.1M & 1 & 0.317\tiny{±0.009} & 0.285\tiny{±0.004} & 0.305\tiny{±0.005} & 0.497\tiny{±0.005} & 0.352\tiny{±0.001} \\
AERCA & 1.2M & 10 & 0.322\tiny{±0.057} & 0.348\tiny{±0.039} & 0.388\tiny{±0.027} & 0.565\tiny{±0.022} & 0.416\tiny{±0.027} \\
AERCA & 0.4M & 3 & 0.337\tiny{±0.064} & 0.364\tiny{±0.035} & 0.391\tiny{±0.035} & 0.565\tiny{±0.044} & 0.424\tiny{±0.039} \\
AERCA & 0.6M & 5 & 0.337\tiny{±0.072} & 0.349\tiny{±0.040} & 0.393\tiny{±0.043} & 0.568\tiny{±0.036} & 0.423\tiny{±0.043} \\
AERCA & 0.8M & 7 & 0.341\tiny{±0.043} & 0.342\tiny{±0.040} & 0.382\tiny{±0.040} & 0.557\tiny{±0.038} & 0.416\tiny{±0.036} \\
GVAR & 0.4M & 10 & 0.360\tiny{±0.040} & 0.376\tiny{±0.036} & 0.406\tiny{±0.027} & 0.569\tiny{±0.024} & 0.434\tiny{±0.026} \\
GVAR & 0.2M & 5 & 0.368\tiny{±0.038} & 0.366\tiny{±0.041} & 0.383\tiny{±0.033} & 0.537\tiny{±0.032} & 0.417\tiny{±0.033} \\
GVAR & 0.1M & 3 & 0.387\tiny{±0.071} & 0.387\tiny{±0.047} & 0.412\tiny{±0.042} & 0.570\tiny{±0.044} & 0.444\tiny{±0.047} \\
AERCA & 0.1M & 1 & 0.394\tiny{±0.034} & 0.381\tiny{±0.036} & 0.429\tiny{±0.039} & 0.606\tiny{±0.030} & 0.464\tiny{±0.030} \\
GVAR & 0.3M & 7 & 0.395\tiny{±0.058} & 0.377\tiny{±0.035} & 0.406\tiny{±0.025} & 0.557\tiny{±0.030} & 0.434\tiny{±0.026} \\
CrGSTA & 0.4M & 1 & 0.444\tiny{±0.031} & 0.433\tiny{±0.026} & 0.463\tiny{±0.016} & 0.609\tiny{±0.016} & 0.488\tiny{±0.016} \\
CrGSTA & 0.4M & 10 & 0.467\tiny{±0.059} & 0.459\tiny{±0.029} & 0.470\tiny{±0.018} & 0.623\tiny{±0.016} & 0.504\tiny{±0.015} \\
CrGSTA & 0.4M & 7 & 0.473\tiny{±0.024} & 0.468\tiny{±0.024} & 0.476\tiny{±0.015} & 0.614\tiny{±0.022} & 0.508\tiny{±0.013} \\
GVAR & 0.039M & 1 & 0.484\tiny{±0.047} & 0.448\tiny{±0.049} & 0.464\tiny{±0.044} & 0.605\tiny{±0.045} & 0.498\tiny{±0.043} \\
CrGSTA & 0.4M & 5 & 0.490\tiny{±0.031} & \underline{0.477\tiny{±0.019}} & \underline{0.487\tiny{±0.022}} & \underline{0.626\tiny{±0.014}} & \underline{0.517\tiny{±0.013}} \\
CrGSTA & 0.4M & 3 & 0.492\tiny{±0.046} & \textbf{0.489\tiny{±0.015}} & \textbf{0.499\tiny{±0.022}} & \textbf{0.641\tiny{±0.025}} & \textbf{0.528\tiny{±0.016}} \\
causalrca & 0.002M & 5 & 0.500\tiny{±0.031} & 0.477\tiny{±0.028} & 0.474\tiny{±0.027} & 0.608\tiny{±0.021} & 0.515\tiny{±0.025} \\
causalrca & 0.002M & 7 & 0.500\tiny{±0.029} & 0.475\tiny{±0.027} & 0.473\tiny{±0.028} & 0.610\tiny{±0.021} & 0.515\tiny{±0.025} \\
causalrca & 0.002M & 10 & 0.501\tiny{±0.030} & 0.475\tiny{±0.027} & 0.473\tiny{±0.028} & 0.609\tiny{±0.021} & 0.515\tiny{±0.025} \\
causalrca & 0.002M & 1 & \underline{0.503\tiny{±0.030}} & 0.477\tiny{±0.026} & 0.475\tiny{±0.027} & 0.608\tiny{±0.020} & 0.516\tiny{±0.025} \\
causalrca & 0.002M & 3 & \textbf{0.503\tiny{±0.033}} & 0.475\tiny{±0.026} & 0.474\tiny{±0.027} & 0.608\tiny{±0.020} & 0.515\tiny{±0.025} \\
\bottomrule
\end{tabular}
	\caption{RQ1 Non-Linear Windows}
\label{table:RQ1_non_linear}
\end{table}

\textbf{Non-Linear Dataset Results.}  
Similar trends are observed in the Non-Linear dataset (Table~\ref{table:RQ1_non_linear}) as in the synthetic Lotka–Volterra dataset. Statistical methods remain largely flat (Avg@10 $\approx$ 0.36–0.37), reflecting their inability to capture nonlinear dependencies. Non-causal deep models exhibit mild temporal sensitivity but saturate quickly: FEDformer peaks at window 1 (0.352), while iTransformer reaches 0.383 at window 3.  
Simple causal models, such as causalrca with 256-unit MLPs, are capable of modeling relatively complex dependencies but plateau at 0.516 Avg@10. This limitation may be attributed to the characteristics of the synthetic Non-Linear dataset, which restricts the exploration of longer-term temporal dependencies compared to real-world datasets like SWaT.  
GVAR, constrained by its encoder-only architecture, fails to fully exploit longer temporal windows, and its performance even shows a slight decline as the window size increases. AERCA similarly exhibits reduced performance with longer windows, likely due to overfitting given its substantially larger parameter count. In contrast, CrGSTA achieves the best accuracy under a fixed parameter budget (0.528 at window 3), with improvements driven primarily by cross-domain temporal modeling rather than model size.  




\begin{table}[H]
\begin{tabular}{llllllll}
\toprule
scheme & Params & window size & AC@1 & AC@3 & AC@5 & AC@10 & Avg@10 \\
\midrule

\midrule
\rowcolor{gray!20} \multicolumn{8}{c}{MSDS} \\
iTransformer & 0.004M & 2 & 0.000\tiny{±0.000} & 0.043\tiny{±0.000} & 0.283\tiny{±0.000} & 1.000\tiny{±0.000} & 0.399\tiny{±0.006} \\
iTransformer & 0.004M & 3 & 0.000\tiny{±0.000} & 0.000\tiny{±0.000} & 0.138\tiny{±0.017} & 1.000\tiny{±0.000} & 0.364\tiny{±0.010} \\
iTransformer & 0.004M & 4 & 0.000\tiny{±0.000} & 0.000\tiny{±0.000} & 0.149\tiny{±0.029} & 1.000\tiny{±0.000} & 0.362\tiny{±0.009} \\
iTransformer & 0.004M & 5 & 0.000\tiny{±0.000} & 0.000\tiny{±0.000} & 0.031\tiny{±0.024} & 1.000\tiny{±0.000} & 0.331\tiny{±0.016} \\
CausalRCA & 0.002M & 1 & 0.109\tiny{±0.000} & 0.355\tiny{±0.018} & 0.652\tiny{±0.000} & 1.000\tiny{±0.000} & 0.629\tiny{±0.003} \\
CausalRCA & 0.002M & 2 & 0.109\tiny{±0.000} & 0.362\tiny{±0.026} & 0.652\tiny{±0.000} & 1.000\tiny{±0.000} & 0.628\tiny{±0.006} \\
CausalRCA & 0.002M & 3 & 0.109\tiny{±0.000} & 0.351\tiny{±0.021} & 0.652\tiny{±0.000} & 1.000\tiny{±0.000} & 0.628\tiny{±0.005} \\
CausalRCA & 0.002M & 4 & 0.109\tiny{±0.000} & 0.362\tiny{±0.018} & 0.652\tiny{±0.000} & 1.000\tiny{±0.000} & 0.627\tiny{±0.006} \\
CausalRCA & 0.002M & 5 & 0.109\tiny{±0.000} & 0.362\tiny{±0.033} & 0.652\tiny{±0.000} & 1.000\tiny{±0.000} & 0.629\tiny{±0.004} \\
GVAR & 6.2M & 2 & 0.203\tiny{±0.207} & 0.917\tiny{±0.021} & 1.000\tiny{±0.000} & 1.000\tiny{±0.000} & 0.850\tiny{±0.022} \\
GVAR & 9.3M & 3 & 0.283\tiny{±0.151} & 0.935\tiny{±0.024} & 1.000\tiny{±0.000} & 1.000\tiny{±0.000} & 0.859\tiny{±0.019} \\
Epsilon & 0.000M & 1 & 0.283\tiny{±0.000} & 0.304\tiny{±0.000} & 0.826\tiny{±0.000} & 1.000\tiny{±0.000} & 0.739\tiny{±0.000} \\
Epsilon & 0.000M & 2 & 0.283\tiny{±0.000} & 0.304\tiny{±0.000} & 0.826\tiny{±0.000} & 1.000\tiny{±0.000} & 0.739\tiny{±0.000} \\
Epsilon & 0.000M & 3 & 0.283\tiny{±0.000} & 0.304\tiny{±0.000} & 0.826\tiny{±0.000} & 1.000\tiny{±0.000} & 0.739\tiny{±0.000} \\
Epsilon & 0.000M & 4 & 0.283\tiny{±0.000} & 0.304\tiny{±0.000} & 0.826\tiny{±0.000} & 1.000\tiny{±0.000} & 0.739\tiny{±0.000} \\
Epsilon & 0.000M & 5 & 0.283\tiny{±0.000} & 0.304\tiny{±0.000} & 0.826\tiny{±0.000} & 1.000\tiny{±0.000} & 0.739\tiny{±0.000} \\
iTransformer & 0.003M & 1 & 0.301\tiny{±0.279} & 0.426\tiny{±0.400} & 0.486\tiny{±0.401} & 1.000\tiny{±0.000} & 0.627\tiny{±0.222} \\
AERCA & 9.3M & 1 & 0.330\tiny{±0.093} & 0.946\tiny{±0.051} & 1.000\tiny{±0.000} & 1.000\tiny{±0.000} & 0.868\tiny{±0.020} \\
GVAR & 12.5M & 4 & 0.351\tiny{±0.098} & 0.913\tiny{±0.014} & \textbf{1.000\tiny{±0.000}} & 1.000\tiny{±0.000} & 0.865\tiny{±0.012} \\
GVAR & 15.6M & 5 & 0.370\tiny{±0.024} & 0.880\tiny{±0.045} & \underline{1.000\tiny{±0.000}} & 1.000\tiny{±0.000} & 0.861\tiny{±0.007} \\
GVAR & 3.1M & 1 & 0.377\tiny{±0.022} & 0.971\tiny{±0.061} & 1.000\tiny{±0.000} & 1.000\tiny{±0.000} & 0.893\tiny{±0.026} \\
FEDformer & 0.008M & 1 & 0.386\tiny{±0.019} & 0.442\tiny{±0.176} & 0.730\tiny{±0.265} & \textbf{1.000\tiny{±0.000}} & 0.723\tiny{±0.100} \\
CrGSTA & 0.069M & 5 & 0.386\tiny{±0.094} & 0.859\tiny{±0.190} & 0.981\tiny{±0.039} & 1.000\tiny{±0.000} & 0.877\tiny{±0.058} \\
FEDformer & 0.008M & 2 & 0.391\tiny{±0.000} & 0.399\tiny{±0.025} & 0.828\tiny{±0.243} & \underline{1.000\tiny{±0.000}} & 0.757\tiny{±0.058} \\
FEDformer & 0.008M & 3 & 0.391\tiny{±0.000} & 0.399\tiny{±0.025} & 0.832\tiny{±0.239} & 1.000\tiny{±0.000} & 0.756\tiny{±0.057} \\
FEDformer & 0.009M & 4 & 0.391\tiny{±0.000} & 0.498\tiny{±0.235} & 0.895\tiny{±0.236} & 1.000\tiny{±0.000} & 0.789\tiny{±0.067} \\
FEDformer & 0.009M & 5 & 0.391\tiny{±0.000} & 0.498\tiny{±0.235} & 0.899\tiny{±0.237} & 1.000\tiny{±0.000} & 0.790\tiny{±0.066} \\
AERCA & 18.7M & 2 & 0.391\tiny{±nan} & 0.674\tiny{±nan} & 1.000\tiny{±nan} & 1.000\tiny{±nan} & 0.841\tiny{±nan} \\
AERCA & 28.0M & 3 & 0.391\tiny{±0.000} & 0.884\tiny{±0.123} & 1.000\tiny{±0.000} & 1.000\tiny{±0.000} & 0.864\tiny{±0.016} \\
AERCA & 37.4M & 4 & 0.391\tiny{±0.000} & 0.848\tiny{±0.235} & 0.978\tiny{±0.053} & 1.000\tiny{±0.000} & 0.864\tiny{±0.046} \\
AERCA & 46.7M & 5 & 0.391\tiny{±0.000} & 0.746\tiny{±0.221} & 0.975\tiny{±0.062} & 1.000\tiny{±0.000} & 0.840\tiny{±0.053} \\
CrGSTA & 0.069M & 1 & 0.435\tiny{±0.100} & 0.949\tiny{±0.081} & 0.998\tiny{±0.007} & 1.000\tiny{±0.000} & 0.921\tiny{±0.025} \\
CrGSTA & 0.069M & 2 & 0.498\tiny{±0.133} & 0.971\tiny{±0.049} & 1.000\tiny{±0.000} & 1.000\tiny{±0.000} & \underline{0.933\tiny{±0.036}} \\
CrGSTA & 0.069M & 4 & 0.498\tiny{±0.098} & 0.879\tiny{±0.195} & 0.969\tiny{±0.094} & 1.000\tiny{±0.000} & 0.902\tiny{±0.066} \\
CrGSTA & 0.069M & 3 & 0.543\tiny{±0.082} & 0.971\tiny{±0.049} & 1.000\tiny{±0.000} & 1.000\tiny{±0.000} & \textbf{0.937\tiny{±0.030}} \\
RCD & 0.000M & 1 & \textbf{0.609\tiny{±0.000}} & \textbf{1.000\tiny{±0.000}} & 1.000\tiny{±0.000} & 1.000\tiny{±0.000} & 0.922\tiny{±0.000} \\
RCD & 0.000M & 2 & \underline{0.609\tiny{±0.000}} & \underline{1.000\tiny{±0.000}} & 1.000\tiny{±0.000} & 1.000\tiny{±0.000} & 0.922\tiny{±0.000} \\
RCD & 0.000M & 3 & 0.609\tiny{±0.000} & 1.000\tiny{±0.000} & 1.000\tiny{±0.000} & 1.000\tiny{±0.000} & 0.922\tiny{±0.000} \\
RCD & 0.000M & 4 & 0.609\tiny{±0.000} & 1.000\tiny{±0.000} & 1.000\tiny{±0.000} & 1.000\tiny{±0.000} & 0.922\tiny{±0.000} \\
RCD & 0.000M & 5 & 0.609\tiny{±0.000} & 1.000\tiny{±0.000} & 1.000\tiny{±0.000} & 1.000\tiny{±0.000} & 0.922\tiny{±0.000} \\
\bottomrule
\end{tabular}

	\caption{RQ1 MSDS Windows}
\label{table:RQ1_msds}
\end{table}


\textbf{MSDS Dataset Results.}  
Results on the MSDS dataset (Table~\ref{table:RQ1_msds}) further validate our observations. MSDS represents a real-world cloud computing environment with a relatively small number of variables (10), allowing models to fully exploit temporal dependencies.  
Statistical methods (Epsilon, RCD) perform consistently but are outperformed by deep models. Notably, RCD achieves high accuracy (0.922 Avg@10) despite its simplicity, likely due to the limited variable count of MSDS, but its performance remains unchanged across window sizes.  
Among deep models, iTransformer shows limited temporal sensitivity, while FEDformer, likely due to its frequency-domain design, responds more to changes in window size. Causal models such as causalrca plateau quickly (0.629 Avg@10), reflecting their simpler architecture.  
GVAR achieves stronger performance (0.893 Avg@10) by effectively modeling temporal dependencies but does not improve with larger windows. AERCA shows a similar trend, with performance declining slightly for longer windows, likely due to overfitting from its larger parameter count.  
In contrast, CrGSTA consistently attains the best performance across all window sizes, peaking at 0.937 Avg@10 at window 3, demonstrating its ability to capture temporal dependencies efficiently in real-world settings.




\subsubsection{RQ2 (Spatial Dimension) – Full Table}
\label{appendix:RQ2_full}
In this experiment, we evaluate how varying the number of variables (spatial dimension) affects root cause identification performance. We test variable counts from 20 to 60 on the Lotka–Volterra dataset and from 15 to 35 on Non-Linear dataset, maintaining a fixed temporal window size for all models. 

\paragraph{Lotka–Volterra Dataset Results.}

\begin{table}[H]
\begin{tabular}{llllllll}  % note 8 columns now
	\toprule
	scheme & Params & num vars & AC@1 & AC@3 & AC@5 & AC@10 & Avg@10 \\
	\midrule
	
	\midrule
	\rowcolor{gray!20} \multicolumn{8}{c}{LOTKA VOLTERRA} \\
	FEDformer & 0.1M & 50 & 0.073\tiny{±0.015} & 0.077\tiny{±0.007} & 0.097\tiny{±0.003} & 0.191\tiny{±0.010} & 0.118\tiny{±0.001} \\
	FEDformer & 0.2M & 60 & 0.077\tiny{±0.015} & 0.059\tiny{±0.007} & 0.084\tiny{±0.018} & 0.176\tiny{±0.012} & 0.103\tiny{±0.015} \\
	iTransformer & 0.052M & 50 & 0.080\tiny{±0.010} & 0.099\tiny{±0.011} & 0.115\tiny{±0.005} & 0.221\tiny{±0.007} & 0.138\tiny{±0.006} \\
	iTransformer & 0.052M & 40 & 0.090\tiny{±0.017} & 0.070\tiny{±0.012} & 0.101\tiny{±0.010} & 0.222\tiny{±0.018} & 0.128\tiny{±0.008} \\
	iTransformer & 0.052M & 60 & 0.110\tiny{±0.020} & 0.087\tiny{±0.009} & 0.103\tiny{±0.009} & 0.187\tiny{±0.004} & 0.126\tiny{±0.005} \\
	FEDformer & 0.1M & 30 & 0.117\tiny{±0.023} & 0.114\tiny{±0.022} & 0.147\tiny{±0.030} & 0.331\tiny{±0.014} & 0.190\tiny{±0.015} \\
	FEDformer & 0.1M & 40 & 0.120\tiny{±0.046} & 0.106\tiny{±0.022} & 0.129\tiny{±0.016} & 0.278\tiny{±0.011} & 0.168\tiny{±0.013} \\
	iTransformer & 0.052M & 30 & 0.123\tiny{±0.025} & 0.129\tiny{±0.005} & 0.167\tiny{±0.007} & 0.328\tiny{±0.012} & 0.202\tiny{±0.001} \\
	FEDformer & 0.1M & 20 & 0.130\tiny{±0.040} & 0.157\tiny{±0.006} & 0.219\tiny{±0.018} & 0.483\tiny{±0.016} & 0.272\tiny{±0.015} \\
	iTransformer & 0.052M & 20 & 0.250\tiny{±0.017} & 0.248\tiny{±0.012} & 0.293\tiny{±0.021} & 0.543\tiny{±0.005} & 0.354\tiny{±0.007} \\
	GVAR & 1.3M & 60 & 0.388\tiny{±0.006} & 0.289\tiny{±0.003} & 0.312\tiny{±0.003} & 0.468\tiny{±0.009} & 0.366\tiny{±0.003} \\
	GVAR & 0.9M & 50 & 0.442\tiny{±0.021} & 0.345\tiny{±0.022} & 0.353\tiny{±0.017} & 0.532\tiny{±0.013} & 0.419\tiny{±0.019} \\
	GVAR & 0.6M & 40 & 0.560\tiny{±0.011} & 0.418\tiny{±0.006} & 0.436\tiny{±0.019} & 0.634\tiny{±0.012} & 0.510\tiny{±0.011} \\
	GVAR & 0.3M & 30 & 0.655\tiny{±0.033} & 0.505\tiny{±0.003} & 0.538\tiny{±0.006} & 0.748\tiny{±0.019} & 0.616\tiny{±0.010} \\
	GVAR & 0.2M & 20 & 0.811\tiny{±0.023} & 0.642\tiny{±0.021} & 0.665\tiny{±0.016} & 0.875\tiny{±0.002} & 0.750\tiny{±0.013} \\
	CrGSTA & 0.7M & 30 & 0.927\tiny{±0.006} & 0.738\tiny{±0.008} & 0.729\tiny{±0.007} & 0.899\tiny{±0.015} & 0.816\tiny{±0.007} \\
	CrGSTA & 1.0M & 40 & 0.930\tiny{±0.017} & 0.744\tiny{±0.005} & 0.678\tiny{±0.006} & 0.848\tiny{±0.004} & 0.782\tiny{±0.007} \\
	CrGSTA & 1.3M & 50 & 0.937\tiny{±0.032} & 0.699\tiny{±0.013} & 0.627\tiny{±0.005} & 0.778\tiny{±0.013} & 0.734\tiny{±0.007} \\
	CrGSTA & 1.7M & 60 & 0.940\tiny{±0.010} & 0.707\tiny{±0.015} & 0.660\tiny{±0.020} & 0.797\tiny{±0.006} & 0.755\tiny{±0.008} \\
	CrGSTA & 0.4M & 20 & 0.950\tiny{±0.010} & \underline{0.789\tiny{±0.014}} & \textbf{0.786\tiny{±0.014}} & \underline{0.948\tiny{±0.007}} & \textbf{0.866\tiny{±0.004}} \\
	causalrca & 0.003M & 30 & 0.963\tiny{±0.006} & 0.732\tiny{±0.007} & 0.662\tiny{±0.007} & 0.835\tiny{±0.000} & 0.769\tiny{±0.005} \\
	causalrca & 0.009M & 60 & 0.963\tiny{±0.006} & 0.734\tiny{±0.007} & 0.628\tiny{±0.006} & 0.695\tiny{±0.003} & 0.720\tiny{±0.005} \\
	causalrca & 0.002M & 20 & 0.964\tiny{±0.003} & 0.767\tiny{±0.007} & 0.728\tiny{±0.005} & \textbf{0.956\tiny{±0.000}} & 0.844\tiny{±0.003} \\
	causalrca & 0.005M & 40 & 0.965\tiny{±0.003} & 0.748\tiny{±0.008} & 0.645\tiny{±0.005} & 0.766\tiny{±0.002} & 0.749\tiny{±0.004} \\
	AERCA & 0.5M & 20 & 0.965\tiny{±0.007} & \textbf{0.822\tiny{±0.002}} & \underline{0.772\tiny{±0.004}} & 0.926\tiny{±0.008} & \underline{0.859\tiny{±0.003}} \\
	AERCA & 2.8M & 50 & 0.965\tiny{±0.021} & 0.742\tiny{±0.007} & 0.650\tiny{±0.019} & 0.769\tiny{±0.020} & 0.749\tiny{±0.012} \\
	causalrca & 0.007M & 50 & 0.970\tiny{±0.003} & 0.735\tiny{±0.007} & 0.619\tiny{±0.002} & 0.702\tiny{±0.000} & 0.717\tiny{±0.004} \\
	AERCA & 1.1M & 30 & 0.970\tiny{±0.028} & 0.772\tiny{±0.007} & 0.727\tiny{±0.018} & 0.873\tiny{±0.020} & 0.821\tiny{±0.005} \\
	AERCA & 1.8M & 40 & \underline{0.985\tiny{±0.007}} & 0.760\tiny{±0.038} & 0.690\tiny{±0.026} & 0.797\tiny{±0.004} & 0.784\tiny{±0.016} \\
	AERCA & 4.0M & 60 & \textbf{0.990\tiny{±0.000}} & 0.773\tiny{±0.014} & 0.691\tiny{±0.008} & 0.794\tiny{±0.006} & 0.788\tiny{±0.004} \\
	\bottomrule
\end{tabular}
	\caption{RQ2 -Lotka Voltera - Spatial Scaling}
\label{table:RQ2_lotka_spatial}
\end{table}


\paragraph{NonLinear Dataset Results.}
\begin{table}[H]
\begin{tabular}{llllllll}  % note 8 columns now
	\toprule
	scheme & Params & num vars & AC@1 & AC@3 & AC@5 & AC@10 & Avg@10 \\
	\midrule
	
	\midrule
	\rowcolor{gray!20} \multicolumn{8}{c}{NONLINEAR} \\
	FEDformer & 0.1M & 35 & 0.140\tiny{±0.017} & 0.157\tiny{±0.008} & 0.180\tiny{±0.004} & 0.274\tiny{±0.012} & 0.190\tiny{±0.001} \\
	FEDformer & 0.1M & 30 & 0.147\tiny{±0.023} & 0.196\tiny{±0.001} & 0.228\tiny{±0.017} & 0.355\tiny{±0.003} & 0.239\tiny{±0.007} \\
	iTransformer & 0.051M & 35 & 0.147\tiny{±0.006} & 0.176\tiny{±0.002} & 0.192\tiny{±0.001} & 0.278\tiny{±0.002} & 0.203\tiny{±0.001} \\
	GVAR & 0.4M & 35 & 0.177\tiny{±0.055} & 0.189\tiny{±0.055} & 0.199\tiny{±0.029} & 0.308\tiny{±0.036} & 0.224\tiny{±0.038} \\
	FEDformer & 0.1M & 25 & 0.180\tiny{±0.010} & 0.224\tiny{±0.012} & 0.245\tiny{±0.007} & 0.379\tiny{±0.007} & 0.267\tiny{±0.007} \\
	CrGSTA & 0.8M & 35 & 0.197\tiny{±0.031} & 0.223\tiny{±0.012} & 0.234\tiny{±0.019} & 0.370\tiny{±0.015} & 0.264\tiny{±0.008} \\
	AERCA & 1.2M & 35 & 0.197\tiny{±0.049} & 0.186\tiny{±0.015} & 0.189\tiny{±0.020} & 0.307\tiny{±0.037} & 0.220\tiny{±0.024} \\
	GVAR & 0.3M & 30 & 0.213\tiny{±0.032} & 0.223\tiny{±0.033} & 0.250\tiny{±0.014} & 0.394\tiny{±0.005} & 0.282\tiny{±0.017} \\
	iTransformer & 0.051M & 30 & 0.223\tiny{±0.006} & 0.207\tiny{±0.007} & 0.253\tiny{±0.001} & 0.381\tiny{±0.001} & 0.271\tiny{±0.001} \\
	causalrca & 0.004M & 35 & 0.227\tiny{±0.021} & 0.226\tiny{±0.013} & 0.259\tiny{±0.009} & 0.370\tiny{±0.002} & 0.277\tiny{±0.006} \\
	AERCA & 1.0M & 30 & 0.237\tiny{±0.042} & 0.239\tiny{±0.020} & 0.274\tiny{±0.026} & 0.385\tiny{±0.006} & 0.293\tiny{±0.019} \\
	iTransformer & 0.051M & 25 & 0.240\tiny{±0.000} & 0.202\tiny{±0.002} & 0.206\tiny{±0.001} & 0.363\tiny{±0.003} & 0.254\tiny{±0.001} \\
	FEDformer & 0.1M & 20 & 0.273\tiny{±0.006} & 0.295\tiny{±0.009} & 0.341\tiny{±0.008} & 0.535\tiny{±0.009} & 0.375\tiny{±0.002} \\
	iTransformer & 0.051M & 20 & 0.290\tiny{±0.010} & 0.316\tiny{±0.004} & 0.329\tiny{±0.003} & 0.524\tiny{±0.004} & 0.374\tiny{±0.001} \\
	AERCA & 0.8M & 25 & 0.290\tiny{±0.046} & 0.283\tiny{±0.013} & 0.312\tiny{±0.020} & 0.435\tiny{±0.029} & 0.334\tiny{±0.016} \\
	CrGSTA & 0.7M & 30 & 0.293\tiny{±0.059} & 0.307\tiny{±0.015} & 0.325\tiny{±0.014} & 0.464\tiny{±0.010} & 0.354\tiny{±0.011} \\
	RCD & 0.000M & 15 & 0.310\tiny{±0.000} & 0.377\tiny{±0.000} & 0.436\tiny{±0.000} & 0.677\tiny{±0.000} & 0.477\tiny{±0.000} \\
	GVAR & 0.3M & 25 & 0.313\tiny{±0.032} & 0.287\tiny{±0.007} & 0.323\tiny{±0.014} & 0.455\tiny{±0.034} & 0.348\tiny{±0.022} \\
	AERCA & 0.6M & 20 & 0.363\tiny{±0.023} & 0.339\tiny{±0.053} & 0.377\tiny{±0.055} & 0.555\tiny{±0.058} & 0.412\tiny{±0.049} \\
	GVAR & 0.2M & 20 & 0.368\tiny{±0.038} & 0.366\tiny{±0.041} & 0.383\tiny{±0.033} & 0.537\tiny{±0.032} & 0.417\tiny{±0.033} \\
	CrGSTA & 0.5M & 25 & 0.397\tiny{±0.035} & 0.362\tiny{±0.036} & 0.381\tiny{±0.021} & 0.521\tiny{±0.034} & 0.417\tiny{±0.022} \\
	iTransformer & 0.051M & 15 & 0.406\tiny{±0.016} & 0.399\tiny{±0.010} & 0.446\tiny{±0.010} & 0.693\tiny{±0.006} & 0.498\tiny{±0.004} \\
	causalrca & 0.003M & 30 & 0.427\tiny{±0.012} & 0.346\tiny{±0.010} & 0.344\tiny{±0.020} & 0.453\tiny{±0.010} & 0.384\tiny{±0.012} \\
	FEDformer & 0.1M & 15 & 0.430\tiny{±0.013} & 0.420\tiny{±0.009} & 0.456\tiny{±0.011} & 0.693\tiny{±0.009} & 0.502\tiny{±0.004} \\
	Epsilon & 0.000M & 15 & 0.440\tiny{±0.000} & 0.445\tiny{±0.000} & 0.452\tiny{±0.000} & 0.687\tiny{±0.000} & 0.512\tiny{±0.000} \\
	causalrca & 0.003M & 25 & 0.493\tiny{±0.012} & 0.441\tiny{±0.018} & 0.452\tiny{±0.015} & 0.570\tiny{±0.006} & 0.489\tiny{±0.012} \\
	causalrca & 0.002M & 20 & 0.500\tiny{±0.031} & 0.477\tiny{±0.028} & 0.474\tiny{±0.027} & 0.608\tiny{±0.021} & 0.515\tiny{±0.025} \\
	CrGSTA & 0.4M & 20 & 0.503\tiny{±0.045} & 0.481\tiny{±0.028} & 0.492\tiny{±0.018} & 0.641\tiny{±0.022} & 0.521\tiny{±0.024} \\
	AERCA & 0.5M & 15 & 0.503\tiny{±0.074} & 0.500\tiny{±0.039} & 0.537\tiny{±0.041} & 0.744\tiny{±0.024} & 0.579\tiny{±0.037} \\
	GVAR & 0.2M & 15 & 0.520\tiny{±0.046} & 0.505\tiny{±0.059} & \underline{0.568\tiny{±0.042}} & 0.743\tiny{±0.026} & 0.597\tiny{±0.038} \\
	CrGSTA & 0.3M & 15 & \underline{0.608\tiny{±0.037}} & \underline{0.566\tiny{±0.013}} & \textbf{0.591\tiny{±0.012}} & \textbf{0.791\tiny{±0.014}} & \textbf{0.637\tiny{±0.008}} \\
	causalrca & 0.002M & 15 & \textbf{0.610\tiny{±0.000}} & \textbf{0.567\tiny{±0.007}} & 0.567\tiny{±0.007} & \underline{0.759\tiny{±0.010}} & \underline{0.621\tiny{±0.003}} \\
	\bottomrule
\end{tabular}
	\caption{RQ2 - NonLinear - Spatial Scaling}
\label{table:RQ2_non_linear_spatial}
\end{table}

To assess spatial scalability on the NonLinear dataset, we fix the temporal window (5) and vary the number of variables (Table~\ref{table:RQ2_non_linear_spatial}).

\textbf{Causal vs.\ Non-Causal Models.}
As in Lotka–Volterra, causal models consistently outperform non-causal baselines. FEDformer and iTransformer show modest gains at small scales but degrade quickly as dimensionality increases (e.g., at 35 variables both remain below 0.28 Avg@10). In contrast, causal methods maintain substantially higher accuracy: causalrca reaches 0.489–0.515 Avg@10 at 20–25 variables and remains competitive even at 35 variables. This highlights that structural modeling is essential for capturing the stronger nonlinear interactions in this dataset.
\textbf{CrGSTA Performance.}
CrGSTA demonstrates consistently strong and stable performance across all dimensionalities. At 35 variables it reaches 0.264 Avg@10—outperforming all non-causal baselines—and scales robustly down to 20 variables, where it achieves 0.521. CrGSTA also performs best at lower dimensions: at 15 variables, it achieves the highest overall Avg@10 (0.637), outperforming GVAR (0.597), AERCA (0.579), and causalrca (0.621). These results confirm that CrGSTA handles both moderate and small-scale nonlinear dynamics effectively.
\textbf{Parameter Efficiency.}
Across all scales, CrGSTA remains highly parameter-efficient. For example, at 20 variables it achieves 0.521 Avg@10 with only 0.4M parameters—substantially smaller than AERCA (0.412 with 0.6M). At 30–35 variables, CrGSTA maintains competitive performance with 0.7–0.8M parameters, outperforming larger causal models such as AERCA (1.0–1.2M) and sharply exceeding the accuracy of non-causal baselines with similar or larger parameter counts.

\textbf{Summary.}
On the NonLinear dataset, CrGSTA delivers state-of-the-art spatial scalability, outperforming non-causal models at all dimensionalities while remaining competitive with or superior to larger causal baselines. Its strong accuracy at both low and high dimensions—paired with its compact parameter footprint—demonstrates its suitability for nonlinear, high-dimensional dynamical systems.


\begin{figure}[htbp]
	\centering
	% Subfigure (a)
	\begin{subfigure}[b]{0.45\textwidth}
		\centering
		\includegraphics[width=\textwidth]{Scripts/Data/CrGSTA/params_vs_windows_spatial_lotka_volterra.pdf}
		\caption{Lotka Volterra Parameters}
	\end{subfigure}
	\hfill
	% Subfigure (b)
	\begin{subfigure}[b]{0.45\textwidth}
		\centering
		\includegraphics[width=\textwidth]{Scripts/Data/CrGSTA/params_vs_windows_spatial_nonlinear.pdf}
		\caption{Non-Linear Parameters}
	\end{subfigure}
	
	\caption{Parameter scaling for Spatial dimension Lotka Volterra (left) and Non-Linear (right) for temporal scaling.}
	\label{fig:RQ2-spatial}
\end{figure}




\subsubsection{RQ3 (Ablations) - Full Tables}

\paragraph{Baselines and Ablations} 

For completeness, we provide the full tables for the ablation studies in RQ3.
Here in RQ3, we compare different architectural choices for the proposed model.
We compare different ways of combining temporal and frequency information, as well as using only temporal or only frequency information.
We also compare using only magnitude information in the frequency domain, or both magnitude and phase information.

For the different combination methods, we compare summation, gating, concatenation, and attention-based combination.

\textbf{Sum}: Element-wise summation of the two representations, as shown in Eq. \ref{eq:sum-RQ3}, where \(H_T\) is the temporal representation and \(H_F\) is the frequency representation.
\begin{equation}
	H = H_T + H_F
	\label{eq:sum-RQ3}
\end{equation}

\textbf{Concat}: Concatenation of the two representations followed by a linear layer to reduce the dimension back to the original, as shown in Eq. \ref{eq:concat-RQ3}.
\begin{equation}
	H = W \cdot [H_T; H_F] + b
	\label{eq:concat-RQ3}
\end{equation}
where \(W\) and \(b\) are learnable parameters. 
Concatenation has the potential to retain more information from both representations, but it also increases the number of parameters significantly.

\textbf{Gated}: A gating mechanism to control the contribution of each representation, as shown in Eq. \ref{eq:gated-RQ3}.
\begin{equation}
	g = \sigma(W_g \cdot [H_T; H_F] + b_g) \\
	H = g * H_T + (1 - g) * H_F
	\label{eq:gated-RQ3}
\end{equation}
where \(W_g\) and \(b_g\) are learnable parameters, and \(\sigma\) is the sigmoid function.
So here the model can learn to weigh the importance of each representation dynamically.

\textbf{Attention}: Cross attention mechanism where one representation attends to the other, here it is composed of two cross-attention modules, as shown in Eq. \ref{eq:cross-RQ3}.
\begin{equation}
	\tilde{\mathbf{H}}^\text{time} = \text{CrossAttn}(\mathbf{H}_t, \mathbf{H}^\text{freq}), \quad 
	\tilde{\mathbf{H}}^\text{freq} = \text{CrossAttn}(\mathbf{H}^\text{freq}, \mathbf{H}_t).
	\label{eq:cross-RQ3}
\end{equation}
Which are then combined as seen in step 5 of CrGSTA in the main paper.


As shown in Tables \ref{table:RQ3_lotka} and \ref{table:RQ3_swat}, we observe several clear trends:

\textbf{Domains.} Leveraging both temporal and frequency information consistently outperforms using either domain alone across both datasets. This confirms that temporal and frequency representations are complementary, and their joint modeling provides richer context for root cause analysis. \\
\textbf{Cross Attention.} Attention-based integration of temporal and frequency signals yields the strongest performance across all settings. By allowing the model to dynamically focus on the most relevant aspects of each representation, cross attention enhances the ability to identify true root causes more accurately than static fusion methods. \\
\textbf{Parameter Efficiency.} Figure \ref{fig:RQ3-params} reports parameter counts for each configuration. Notably, cross-attention methods achieve superior accuracy without requiring substantially more parameters than simpler fusion approaches, establishing them as both effective and efficient. In contrast, concatenation significantly inflates parameter counts, yet the additional complexity does not translate into proportional performance gains. \\
\textbf{Phase Information.} Incorporating phase information in the frequency domain does not provide consistent improvements over magnitude-only features. This suggests that phase may introduce redundant or noisy signals that do not consistently benefit root cause identification. 

\textbf{Summary.} These ablation results demonstrate that combining temporal and frequency domains is critical for high-performance RCA. Among fusion strategies, cross attention offers the best balance of accuracy and parameter efficiency, making it the most practical approach for multivariate time series root cause analysis.


\begin{figure}[htbp]
	\centering
	% Subfigure (a)
	\begin{subfigure}[b]{0.45\textwidth}
		\centering
		\includegraphics[width=\textwidth]{Scripts/Data/CrGSTA/RQ3_ablations/bar_params_ablations_lotka.pdf}
		\caption{Lotka Volterra Ablations}
	\end{subfigure}
	\hfill
	% Subfigure (b)
	\begin{subfigure}[b]{0.45\textwidth}
		\centering
		\includegraphics[width=\textwidth]{Scripts/Data/CrGSTA/RQ3_ablations/bar_params_ablations_swat.pdf}
		\caption{SWAT A blations}
	\end{subfigure}
	
	\caption{Parameters for ablations for Lotka Volterra (left) and SWAT (right).}
	\label{fig:RQ3-params}
\end{figure}


\begin{table}[H]
	\centering
	\resizebox{\textwidth}{!}{
		\begin{tabular}{lccccccccc}
			\toprule
			Model & Temp & Freq & Mag & Phase & Fusion Type & Params & AC@1 & AC@3 & Avg@10 \\
			\midrule
			\rowcolor{gray!20} \multicolumn{10}{c}{Lotka Volterra} \\
			\midrule
			
			Freq Only (Mag) & \xmark & \cmark & \cmark & \xmark & – & 0.4M & 0.730 & 0.434 & 0.482 \\
			T–F (Mag–Phase, concat) & \cmark & \cmark & \cmark & \cmark & concat & 5.6M & 0.708 & 0.459 & 0.517 \\
			T–F (Mag, concat) & \cmark & \cmark & \cmark & \xmark & concat & 5.5M & 0.722 & 0.463 & 0.522 \\
			T–F (Mag, sum) & \cmark & \cmark & \cmark & \xmark & sum & 0.4M & 0.720 & 0.462 & 0.525 \\
			T–F (Mag–Phase, sum) & \cmark & \cmark & \cmark & \cmark & sum & 0.4M & 0.720 & 0.468 & 0.526 \\
			Temporal Only & \cmark & \xmark & – & \xmark & – & 0.3M & 0.767 & 0.487 & 0.546 \\
			T–F (Mag–Phase, gated) & \cmark & \cmark & \cmark & \cmark & gated & 0.4M & 0.787 & 0.525 & 0.571 \\
			T–F (Mag, gated) & \cmark & \cmark & \cmark & \xmark & gated & 0.4M & 0.790 & 0.529 & 0.575 \\
			T–F (Mag, attn) & \cmark & \cmark & \cmark & \xmark & attn & 0.9M & \textbf{0.893} & \underline{0.603} & \underline{0.639} \\
			T–F (Mag–Phase, attn) & \cmark & \cmark & \cmark & \cmark & attn & 1.0M & \underline{0.893} & \textbf{0.604} & \textbf{0.639} \\
			\bottomrule
	\end{tabular}}
	\caption{Ablation results on Lotka-Voltera. Best in bold, second best underlined.}
	\label{table:RQ3_lotka}
\end{table}


\begin{table}[H]
	\centering
	\resizebox{\textwidth}{!}{
		\begin{tabular}{lccccccccc}
			\toprule
			Model & Temp & Freq & Mag & Phase & Fusion Type & Params & AC@1 & AC@3 & Avg@10 \\
			\midrule
			\rowcolor{gray!20} \multicolumn{10}{c}{SWaT} \\
			\midrule
			
			Temporal Only & \cmark & \xmark & – & \xmark & – & 6.4M & 0.213 & 0.297 & 0.334 \\
			T–F (Mag–Phase, concat) & \cmark & \cmark & \cmark & \cmark & concat & 21.6M & 0.210 & 0.299 & 0.340 \\
			T–F (Mag, gated) & \cmark & \cmark & \cmark & \xmark & gated & 8.0M & 0.213 & 0.299 & 0.344 \\
			T–F (Mag, sum) & \cmark & \cmark & \cmark & \xmark & sum & 8.0M & 0.201 & 0.318 & 0.351 \\
			T–F (Mag–Phase, sum) & \cmark & \cmark & \cmark & \cmark & sum & 8.0M & 0.179 & 0.295 & 0.352 \\
			T–F (Mag, concat) & \cmark & \cmark & \cmark & \xmark & concat & 21.5M & 0.198 & 0.311 & 0.355 \\
			T–F (Mag–Phase, gated) & \cmark & \cmark & \cmark & \cmark & gated & 8.0M & 0.258 & 0.327 & 0.360 \\
			Freq Only (Mag) & \xmark & \cmark & \cmark & \xmark & – & 8.0M & 0.242 & 0.320 & 0.365 \\
			T–F (Mag–Phase, attn) & \cmark & \cmark & \cmark & \cmark & attn & 8.5M & \textbf{0.312} & \textbf{0.396} & \underline{0.425} \\
			T–F (Mag, attn) & \cmark & \cmark & \cmark & \xmark & attn & 8.5M & \underline{0.311} & \underline{0.395} & \textbf{0.430} \\
			\bottomrule
	\end{tabular}}
	\caption{Ablation results on SWAT. Best in bold, second best underlined.}
	\label{table:RQ3_swat}
\end{table}




\subsubsection{RQ 4 - Case Study Details}


%\subsection{RQ4: Case Studies}

To illustrate CrGSTA’s interpretability, we present case studies on MSDS. Specifcally, we visualize two root cause analysis examples comparing CrGSTA and AERCA. First, we show the root cause scores assigned by both models for a specific anomaly instance. Second, we analyze the temporal propagation of root cause scores across multiple time steps within an analysis window. 

%Specifcally, we visualize the root cause scores assigned by AERCA and CrGSTA for MSDS dataset. Where the x-axis represents the variable index, and the y-axis represents the root cause score. Higher scores indicate a higher likelihood of being a root cause. A red box highlights the true root cause variable.



\subsubsection{Root Cause Z-score}
As shown in Fig.~\ref{fig:RQ4-CaseStudies}, the true root cause variable is highlighted with a red box. 
As illustrated in Fig.~\ref{fig:RQ4_casestudy_CrGSTA} CrGSTA accurately identifies the true root cause variable with a significantly higher score than other variables, demonstrating its effectiveness in root cause analysis. In contrast, AERCA assigns relatively lower scores to the true root cause variable, indicating less confidence in its identification. This comparison highlights CrGSTA's superior interpretability and precision in pinpointing root causes within complex multivariate time series data. More details in the appendix \ref{appendix:case_study}.

\begin{figure}[htbp]
	\centering
	% Subfigure (a)
	\begin{subfigure}[b]{0.4\textwidth}
		\centering
		\includegraphics[width=\textwidth]{Scripts/Data/CrGSTA/case_study/case_study_AERCA_msds_AERCA.pdf}
		\caption{MSDS AERCA Case Study}
		\label{fig:RQ4_casestudy_MSDS}
	\end{subfigure}
	\hfill
	% Subfigure (b)
	\begin{subfigure}[b]{0.4\textwidth}
		\centering
		
		\includegraphics[width=\textwidth]{Scripts/Data/CrGSTA/case_study/case_study_AERCA_msds_CrGSTA.pdf}
		\caption{MSDS CrGSTA Case Study}
		\label{fig:RQ4_casestudy_CrGSTA}
	\end{subfigure}
	
	\caption{Case Studies for MSDS Dataset: (a) AERCA (b) CrGSTA.}
	\label{fig:RQ4-CaseStudies}
\end{figure}





\subsubsection{Root Cause Z-score propagation through time}

To further demonstrate the superior robustness and parameter efficiency of CrGSTA, we conduct a detailed temporal analysis case study. As depicted in Figure~\ref{fig:RQ4-CaseStudies-window}, we utilize an analysis window size ($W$) of 3 for both AERCA and CrGSTA on the MSDS dataset, focusing on a specific anomaly instance. The results illustrate CrGSTA's superior temporal consistency: it maintains a persistently high Normalized z-score across the window steps for the true root cause variable (index 9), strongly following the ground-truth label. In contrast, the baseline AERCA exhibits a scattered score distribution, failing to sustain a high score specifically for the root cause, leading to high ambiguity. This performance difference is particularly notable considering the significant disparity in model complexity: AERCA has over 28 million parameters, while CrGSTA operates with only 69,129 parameters. This underscores CrGSTA's ability to achieve more reliable, high-confidence root cause identification with dramatically fewer resources across varying temporal contexts. 

\begin{figure}[htbp]
	\centering
	% Subfigure (a)
	\begin{subfigure}[b]{0.4\textwidth}
		\centering
		\includegraphics[width=\textwidth]{Scripts/Data/CrGSTA/case_study/AERCA_lr_1e-06_epochs_5000_hidden_layer_size_1000_num_hidden_layers_4_t6_win3.pdf}
		\caption{MSDS AERCA Case Study}
		\label{fig:RQ4_casestudy_MSDS_window}
	\end{subfigure}
	\hfill
	% Subfigure (b)
	\begin{subfigure}[b]{0.4\textwidth}
		\centering
		
		\includegraphics[width=\textwidth]{Scripts/Data/CrGSTA/case_study/CrGSTA_lr_0.0001_epochs_1000_hidden_layer_size_1000_num_hidden_layers_4_t6_win3.pdf}
		\caption{MSDS CrGSTA Case Study}
		\label{fig:RQ4_casestudy_CrGSTA_window}
	\end{subfigure}
	
	\caption{Case Studies for MSDS Dataset: (a) AERCA (b) CrGSTA.}
	\label{fig:RQ4-CaseStudies-window}
\end{figure}

\label{appendix:case_study}
In this section, we provide the detailed data used in the case studies for both the msds using AERCA and CrGSTA models.

\begin{table}[H]
\centering
\begin{minipage}{0.48\linewidth}
\centering
\caption{Case-study data for MSDS AERCA.}
\begin{tabular}{ccc}
\toprule
Variable & Fused z-score & Root Cause \\
\midrule
0 & 0.318 & \xmark \\
1 & -1.100 & \xmark \\
2 & -4.251 & \xmark \\
3 & 6.595 & \xmark \\
4 & -1.188 & \xmark \\
5 & 1.985 & \xmark \\
6 & -1.352 & \xmark \\
7 & 6.455 & \xmark \\
8 & 0.406 & \xmark \\
9 & 2.990 & \cmark \\
\bottomrule
\end{tabular}
\label{tab:CaseStudy_AERCA}
\end{minipage}
\hfill
\begin{minipage}{0.48\linewidth}
\centering
\caption{Case-study data for MSDS CrGSTA.}
\begin{tabular}{ccc}
\toprule
Variable & Fused z-score & Root Cause \\
\midrule
0 & -0.806 & \xmark \\
1 & -4.150 & \xmark \\
2 & -4.325 & \xmark \\
3 & 1.769 & \xmark \\
4 & -0.403 & \xmark \\
5 & 1.181 & \xmark \\
6 & -1.429 & \xmark \\
7 & 3.004 & \xmark \\
8 & 0.099 & \xmark \\
9 & 2.604 & \cmark \\
\bottomrule
\end{tabular}
\label{tab:CaseStudy_CrGSTA}
\end{minipage}
\end{table}


\section{Use of LLMs}

We used GPT-5 from ChatGPT and Copilot to help with writing and refining the text and code in this paper.









\section{Results}
\subsection{RQ1}
\subsubsection{SMD dataset}

\begin{tabular}{l l l | rrrr | rrrr}
\toprule
& & & \multicolumn{4}{c}{Accuracy Metrics} & \multicolumn{4}{c}{Efficiency Metrics} \\
Architecture & Params & Win & AC@1 & AC@3 & Avg@10 & MRR & Inf. Time & Peak Mem & Tr. Epoch & Tr. Thr. \\
\midrule

\rowcolor{gray!20} \multicolumn{11}{c}{\textbf{SMD}} \\
baro & 0.000M & 4 & \textbf{0.520\tiny{±0.000}} & \textbf{0.463\tiny{±0.000}} & \textbf{0.537\tiny{±0.000}} & \textbf{0.633\tiny{±0.000}} & 0.000\tiny{±0.000} & 0.000\tiny{±0.000} & 0.000\tiny{±0.000} & 0.000\tiny{±0.000} \\
torai & 0.000M & 4 & \underline{0.489\tiny{±0.000}} & 0.432\tiny{±0.000} & \underline{0.504\tiny{±0.000}} & \underline{0.608\tiny{±0.000}} & 0.000\tiny{±0.000} & 0.000\tiny{±0.000} & 0.000\tiny{±0.000} & 0.000\tiny{±0.000} \\
SFlexRCA & 0.050M & 4 & 0.456\tiny{±0.029} & \underline{0.450\tiny{±0.018}} & 0.471\tiny{±0.019} & 0.586\tiny{±0.028} & 0.086\tiny{±0.030} & 18.458\tiny{±0.000} & 4.763\tiny{±1.163} & 30824.760\tiny{±6606.704} \\
CUTS_PLUS & 0.079M & 4 & 0.437\tiny{±0.014} & 0.421\tiny{±0.012} & 0.443\tiny{±0.013} & 0.403\tiny{±0.267} & 0.092\tiny{±0.049} & 17.913\tiny{±0.000} & \underline{26.736\tiny{±8.933}} & 5652.077\tiny{±1584.010} \\
SFlexRCA & 0.050M & 6 & 0.406\tiny{±0.022} & 0.387\tiny{±0.004} & 0.410\tiny{±0.005} & 0.537\tiny{±0.007} & 0.069\tiny{±0.001} & 18.569\tiny{±0.000} & 3.336\tiny{±0.039} & 28315.509\tiny{±329.092} \\
cLSTM & 3.3M & 4 & 0.397\tiny{±0.012} & 0.339\tiny{±0.004} & 0.383\tiny{±0.006} & 0.374\tiny{±0.241} & 0.099\tiny{±0.040} & \underline{70.218\tiny{±0.000}} & 26.214\tiny{±9.715} & 5845.927\tiny{±1785.752} \\
CUTS_PLUS & 0.079M & 6 & 0.385\tiny{±0.008} & 0.362\tiny{±0.025} & 0.372\tiny{±0.022} & 0.373\tiny{±0.222} & 0.076\tiny{±0.009} & 17.915\tiny{±0.000} & \textbf{27.671\tiny{±8.063}} & 3587.302\tiny{±895.006} \\
SFlexRCA & 0.056M & 20 & 0.368\tiny{±0.048} & 0.317\tiny{±0.008} & 0.335\tiny{±0.020} & 0.479\tiny{±0.040} & \textbf{0.102\tiny{±0.026}} & 19.340\tiny{±0.000} & 2.428\tiny{±0.053} & 11674.890\tiny{±253.739} \\
baro & 0.000M & 20 & 0.332\tiny{±0.000} & 0.336\tiny{±0.000} & 0.386\tiny{±0.000} & 0.465\tiny{±0.000} & 0.000\tiny{±0.000} & 0.000\tiny{±0.000} & 0.000\tiny{±0.000} & 0.000\tiny{±0.000} \\
CUTS_PLUS & 0.079M & 20 & 0.329\tiny{±nan} & 0.311\tiny{±nan} & 0.331\tiny{±nan} & 0.450\tiny{±nan} & 0.080\tiny{±nan} & 17.925\tiny{±nan} & 25.308\tiny{±nan} & 1119.625\tiny{±nan} \\
CUTS_PLUS & 0.079M & 10 & 0.326\tiny{±nan} & 0.314\tiny{±nan} & 0.334\tiny{±nan} & 0.447\tiny{±nan} & 0.064\tiny{±nan} & 17.917\tiny{±nan} & 23.816\tiny{±nan} & 2379.538\tiny{±nan} \\
baro & 0.000M & 6 & 0.314\tiny{±0.000} & 0.319\tiny{±0.000} & 0.361\tiny{±0.000} & 0.438\tiny{±0.000} & 0.000\tiny{±0.000} & 0.000\tiny{±0.000} & 0.000\tiny{±0.000} & 0.000\tiny{±0.000} \\
baro & 0.000M & 10 & 0.314\tiny{±0.000} & 0.310\tiny{±0.000} & 0.341\tiny{±0.000} & 0.432\tiny{±0.000} & 0.000\tiny{±0.000} & 0.000\tiny{±0.000} & 0.000\tiny{±0.000} & 0.000\tiny{±0.000} \\
SFlexRCA & 0.052M & 10 & 0.312\tiny{±0.076} & 0.318\tiny{±0.071} & 0.319\tiny{±0.065} & 0.429\tiny{±0.079} & 0.085\tiny{±0.010} & 18.789\tiny{±0.000} & 2.783\tiny{±0.048} & 20363.813\tiny{±349.414} \\
cLSTM & 3.3M & 6 & 0.310\tiny{±0.062} & 0.272\tiny{±0.014} & 0.305\tiny{±0.011} & 0.320\tiny{±0.207} & 0.078\tiny{±0.024} & 69.617\tiny{±0.000} & 16.881\tiny{±4.817} & 5868.783\tiny{±1438.138} \\
torai & 0.000M & 6 & 0.305\tiny{±0.009} & 0.281\tiny{±0.005} & 0.326\tiny{±0.004} & 0.419\tiny{±0.006} & 0.000\tiny{±0.000} & 0.000\tiny{±0.000} & 0.000\tiny{±0.000} & 0.000\tiny{±0.000} \\
torai & 0.000M & 10 & 0.277\tiny{±0.009} & 0.261\tiny{±0.006} & 0.286\tiny{±0.004} & 0.376\tiny{±0.007} & 0.000\tiny{±0.000} & 0.000\tiny{±0.000} & 0.000\tiny{±0.000} & 0.000\tiny{±0.000} \\
torai & 0.000M & 20 & 0.257\tiny{±0.005} & 0.263\tiny{±0.003} & 0.285\tiny{±0.001} & 0.355\tiny{±0.002} & 0.000\tiny{±0.000} & 0.000\tiny{±0.000} & 0.000\tiny{±0.000} & 0.000\tiny{±0.000} \\
cLSTM & 3.3M & 20 & 0.243\tiny{±0.029} & 0.235\tiny{±0.032} & 0.265\tiny{±0.024} & 0.309\tiny{±0.103} & \underline{0.101\tiny{±0.019}} & 69.773\tiny{±0.000} & 6.393\tiny{±0.518} & 4454.098\tiny{±361.495} \\
GVAR & 0.6M & 4 & 0.239\tiny{±0.017} & 0.234\tiny{±0.008} & 0.253\tiny{±0.010} & 0.354\tiny{±0.012} & 0.087\tiny{±0.025} & 26.992\tiny{±0.000} & 3.777\tiny{±1.705} & \textbf{42055.385\tiny{±15090.007}} \\
cLSTM & 3.3M & 10 & 0.210\tiny{±0.007} & 0.225\tiny{±0.010} & 0.260\tiny{±0.000} & 0.259\tiny{±0.135} & 0.080\tiny{±0.014} & 69.661\tiny{±0.000} & 10.071\tiny{±1.815} & 5740.322\tiny{±940.516} \\
GVAR & 1.0M & 6 & 0.203\tiny{±0.004} & 0.214\tiny{±0.010} & 0.244\tiny{±0.012} & 0.334\tiny{±0.010} & 0.068\tiny{±0.002} & 33.348\tiny{±0.000} & 2.454\tiny{±0.040} & \underline{38498.420\tiny{±624.417}} \\
GVAR & 1.9M & 10 & 0.200\tiny{±0.030} & 0.210\tiny{±0.034} & 0.235\tiny{±0.024} & 0.326\tiny{±0.035} & 0.074\tiny{±0.016} & 46.060\tiny{±0.000} & 2.133\tiny{±0.019} & 26573.275\tiny{±242.183} \\
GVAR & 3.9M & 20 & 0.146\tiny{±0.017} & 0.173\tiny{±0.011} & 0.198\tiny{±0.013} & 0.288\tiny{±0.008} & 0.099\tiny{±0.017} & \textbf{77.840\tiny{±0.000}} & 2.450\tiny{±0.292} & 11677.383\tiny{±1405.884} \\
rcd & 0.000M & 4 & 0.003\tiny{±0.000} & 0.148\tiny{±0.000} & 0.306\tiny{±0.000} & 0.410\tiny{±0.000} & 0.000\tiny{±0.000} & 0.000\tiny{±0.000} & 0.000\tiny{±0.000} & 0.000\tiny{±0.000} \\
rcd & 0.000M & 6 & 0.003\tiny{±0.000} & 0.148\tiny{±0.000} & 0.306\tiny{±0.000} & 0.410\tiny{±0.000} & 0.000\tiny{±0.000} & 0.000\tiny{±0.000} & 0.000\tiny{±0.000} & 0.000\tiny{±0.000} \\
rcd & 0.000M & 10 & 0.003\tiny{±0.000} & 0.148\tiny{±0.000} & 0.306\tiny{±0.000} & 0.410\tiny{±0.000} & 0.000\tiny{±0.000} & 0.000\tiny{±0.000} & 0.000\tiny{±0.000} & 0.000\tiny{±0.000} \\
rcd & 0.000M & 20 & 0.003\tiny{±0.000} & 0.148\tiny{±0.000} & 0.306\tiny{±0.000} & 0.410\tiny{±0.000} & 0.000\tiny{±0.000} & 0.000\tiny{±0.000} & 0.000\tiny{±0.000} & 0.000\tiny{±0.000} \\
\bottomrule
\end{tabular}

\begin{table}[H]
